# Supplementary material for: Mechanics of Next Token Prediction with Self-Attention
Source: arXiv:2403.08081 source file (2024-03-12)
Supplement: Supplementary file 1 [file appendix.tex]

% \begin{appendices}

\subsection{Global convergence: acyclic data}

\begin{lemma} \label{le:corr} Let $\Wm$ be the SVM solution of (\ref{acyc svm}). Suppose Assumptions \ref{assume same corr pred}, \ref{assume loss} and \ref{assume realizable} hold. For any $\pi > 0$, there exists sufficiently large $R \coloneqq R_{\pi}$, such that for any $\W$ with $\tf{\W} \geq R$, we have 
    \begin{equation}
        \bigg \langle \nabla \mathcal{L}(\W), \frac{\W}{\tf{\W}} \bigg \rangle \geq (1 + \pi) \bigg \langle \nabla \mathcal{L}(\W), \frac{\Wm}{\tf{\Wm}} \bigg \rangle
    \end{equation}
\end{lemma}

\begin{proof}
% The proof is similar to Lemma \ref{global des lem} at a high-level. However, we also need to account for the impact of $\W$ besides $\Ws$ in the gradient correlation. The main goal is showing that $\Ws$ is the near-optimal descent direction, thus, $\W$ cannot significantly outperform it.
%
%\ct{Suggestion to change $\Xi\leftarrow\Theta$,  $\ab_i\leftarrow\hb_i$ and $\bar\ab_i\leftarrow\bar\hb_i$ for consistency with local lemmas below}
Let $\Wb=\tf{\Wm}\W/\tf{\W}$, $M=\sup_{i,t}\tf{\x_{it} \xli^\top}$, $\Theta=1/\tf{\Wm}$, $\s_i=\sft{ \X_i\W \xli}$, $\hb_i= \X_i \Wb\xli$, $\bar\hb_i= \X_i \Wm \xli$, $\bgam_i=\X_i\cb_{y_i}$, and similarly, let
\[
\Oc_i:=\{t~\big|~\x_{it}=\eb_{y_i},t\in[T]\}.
\]
Then we have $\gamma:=\bgam_{it}=\alpha+\beta$ for $t\in\Oc_i$, otherwise $\bgamma:=\bgam_{it}=\beta$.

 Repeating the proof of Lemma~\ref{le:negcorr 2} yields that for any $\W'\in\R^{d\times d}$,
\begin{align*}
\li\nabla\Lc(\W),\W'\ri&=\frac{1}{n}\sum_{i=1}^n \ell'_i\cdot \alpha\sum_{t\in\Oc_i}\s_{it}\left(\sum_{t=1}^T(\hb'_{y_i}-\hb'_{it})\s_{it}\right),
\end{align*}
where $\hb'=\X_i\W'\xli$. Since in this theorem, we focus on the acyclic setting, 
\begin{align*}
\li\nabla\Lc(\W),\Wm\ri&=\frac{1}{n}\sum_{i=1}^n \ell'_i\cdot \alpha\sum_{t\in\Oc_i}\s_{it}\left(\sum_{t=1}^T(\bar\hb_{y_i}-\bar\hb_{it})\s_{it}\right),\\
\li\nabla\Lc(\W),\Wb\ri&=\frac{1}{n}\sum_{i=1}^n \ell'_i\cdot \alpha\sum_{t\in\Oc_i}\s_{it}\left(\sum_{t=1}^T(\hb_{y_i}-\hb_{it})\s_{it}\right).
\end{align*}
Let $\bar\Oc_i:=[T]-\Oc_i$,  $\bar\s_i:=\sum_{t\in\Oc_i}\s_{it}$, $\hb_{y_i}-\hb_{it}=b_{it}$ and $\bar\hb_{y_i}-\bar\hb_{it}=a_{it}$. We will then show that 
\[
\frac{1}{n}\sum_{i\in[n],t\in\bar\Oc_i}\bar\s_i\s_{it}b_{it}\leq(1+\pi)\cdot\frac{1}{n}\sum_{i\in[n],t\in\bar\Oc_i}\bar\s_i\s_{it}a_{it}.
\]
Since $\tf{\Wb}=\tf{\Wm}$, \red{there exist $i,t$ such that, $b_{it}-a_{it}\leq-\delta$, and then $\max_{i,t}b_{it}-a_{it}\leq2\tf{\Wm}-\delta$}
\begin{align*}
    \frac{1}{n}\sum_{i\in[n],t\in\bar\Oc_i}\bar\s_i\s_{it}(b_{it}-a_{it})&\leq\max_{i\in[n]}\sum_{t\in\Oc_i}\bar\s_i\s_{it}(2\tf{\Wm}-\delta)-\frac{1}{n}e^{-\bar R\delta}\delta\\
    &\leq Te^{-\bar R(2\tf{\Wm}-\delta)}(2\tf{\Wm}-\delta)-\frac{1}{n}e^{-\bar R\delta}\delta\\
    &=\frac{1}{n}e^{-\bar R\delta}\left(nT(2\tf{\Wm}-\delta)e^{-2(\bar R(\tf{\Wm}-\delta))}-\delta\right).
\end{align*}
Then we can choose sufficiently large $\bar R$ such that 
\[
\frac{1}{n}e^{-\bar R\delta}\left(nT(2\tf{\Wm}-\delta)e^{-2(\bar R(\tf{\Wm}-\delta))}-\delta\right)\leq\pi\Longrightarrow
\]
\end{proof}

\redp{1. Whether we need zero initialization. (no) 2. Whether we need Assumption \ref{assume realizable} (yes) and \ref{assume orth} (no) for the Theorem.}

\begin{lemma} \label{le:corr} Let $\Wm$ be the SVM solution of (\ref{acyc svm}). Suppose Assumption \ref{assume iden}, \ref{assume loss} and \ref{assume realizable} hold. For any $\pi > 0$, With sufficient large $R \coloneqq R_{\pi}$, such that for any $\W$ with $\tf{\W} \geq R$, we have 
    \begin{equation}
        \bigg \langle \nabla \mathcal{L}(\W), \frac{\W}{\tf{\W}} \bigg \rangle \geq (1 + \pi) \bigg \langle \nabla \mathcal{L}(\W), \frac{\Wm}{\tf{\Wm}} \bigg \rangle
    \end{equation}
\end{lemma}
\begin{proof}
First let $\bar{\W} = \tf{\Wm}\W / \tf{\W}, \bar{\hb}_i = \X_i \Wm \xli, \hb_i = \X_i \bar{W}\xli, \bgam_i = \X_i \xli$ and we have $ \gamma_{it} = 1 \text{ for } t\in \Oc \text{ and } \gamma_{it} = 0 \text{ for } t \in \Ocb$ following Assumption \ref{assume same corr pred}. Repeating the proof of Lemma \ref{le:negcorr} gives: 
\begin{equation}
    \begin{split}
        \langle \nabla \mathcal{L}(\W), {\Wm} \rangle 
        % & = 
        % \frac{1}{n} \sum_{i=1}^n \ell' \cdot (1-s_{i1})'s_{i1}' \bigg [\frac{\sum_{t \in O_i} \bar{h}_{it} s_{it}}{\sum_{t \in O_i} s_{it}} - \frac{\sum_{\tau \in \Ocb_i} \bar{h}_{i\tau} s_{i\tau}}{\sum_{\tau \in \Ocb_i} s_{i\tau}} \bigg ] \\ 
        & = \frac{1}{n} \sum_{i=1}^n \ell' \cdot \alpha\left((1 - \sum_{t\in\Oc}s_{it})\sum_{t\in\Oc}s_{it}\right) \left(\bar{h}_{y_i}- \frac{\sum_{t \in \Ocb_i} \bar{h}_{it}s_{it}}{\sum_{t \in \Ocb_i} s_{it}}\right) \\
        \langle \nabla \mathcal{L}(\W), {\Wb} \rangle 
        % \frac{1}{n} \sum_{i=1}^n \ell' \cdot (1-s_{i1}')s_{i1}' \bigg [\frac{\sum_{t \in O_i} h_{it} s_{it}}{\sum_{t \in O_i} s_{it}} - \frac{\sum_{\tau \in \Ocb_i} h_{i\tau} s_{i\tau}}{\sum_{\tau \in \Ocb_i} s_{i\tau}} \bigg ] \\
        & = \frac{1}{n} \sum_{i=1}^n \ell' \cdot \alpha \left((1 - \sum_{t\in\Oc}s_{it})\sum_{t\in\Oc}s_{it}\right)\left( {h}_{y_i}- \frac{\sum_{t \in \Ocb_i}{h}_{it}s_{it}}{\sum_{t \in \Ocb_i} s_{it}}\right)\\
    \end{split}
\end{equation}
Without the loss of generality, we focus on the input $(\X, y)$ and drop the subscript $i$. We wish to prove that
\begin{equation} \label{eq:mm1}
   (1+\pi) \cdot \left(\bar{h}_{y}- \frac{\sum_{t \in \Ocb} \bar{h}_{t}s_{t}}{\sum_{t \in \Ocb} s_{t}}\right) \geq  {h}_{y}- \frac{\sum_{t \in \Ocb}{h}_{t}s_{t}}{\sum_{t \in \Ocb} s_{t}}
\end{equation}
% Suppose $x_{it} = \eb_k$, it is equivalent to prove:
% \begin{equation}
% \begin{split}
%    (1+\pi) \cdot & \left(\sum_{k\in \Xs_i, k \neq y} (\bar\h_{iy}-\bar\h_{ik})s_{ik}\right) \geq \left(\sum_{k\in \Xs_i, k \neq y}(\h_{iy}-\h_{ik})s_{ik}\right) \\ 
%    s_{ik} &= \frac{\eb_k^{\top}\W\eb_k}{\sum_{j \in \Xs_i}|n_{ij}|\eb_j^{\top}\W\eb_j}
% \end{split}
% \end{equation}
% where $|n_{ij}|$ is the number of tokens in $\Xs_i$ that equals $\eb_j$.\\
\textbf{Case 1: } $\tf{\bar{\W} - \Wm} \leq \epsilon \coloneqq \pi / (2M) $. In this case, for any token, we can show that
\begin{equation}
    |\h_t - \bar{\h}_t| = |x_t^{\top}(\bar{\W} - \Wm)x_T|  \leq M \tf{\bar{\W} - \Wm} \leq M \epsilon
\end{equation}
As a result, we get
\begin{equation}\label{eq:imm1}
\bar{h}_{y}- \frac{\sum_{t \in \Ocb} \bar{h}_{t}s_{t}}{\sum_{t \in \Ocb} s_{t}} \geq {h}_{y}- \frac{\sum_{t \in \Ocb}{h}_{t}s_{t}}{\sum_{t \in \Ocb} s_{t}} - 2M\epsilon 
= {h}_{y}- \frac{\sum_{t \in \Ocb}{h}_{t}s_{t}}{\sum_{t \in \Ocb} s_{t}}  - \pi
\end{equation}
Moreover, recall in Lemma \ref{le:negcorr}, for the solution of \eqref{acyc svm} we have:
\begin{equation} \label{eq:imm2}
\bar{h}_{y}- \frac{\sum_{t \in \Ocb} \bar{h}_{t}s_{t}}{\sum_{t \in \Ocb} s_{t}}  \geq \bar{h}_{y} - \max_{t \in \Ocb} \bar{h}_{t} \geq 1
\end{equation} 
Then we obtain the following using \eqref{eq:imm1} and \eqref{eq:imm2}: 
\begin{equation}
   (1+\pi) \cdot  \left( \bar{h}_{y}- \frac{\sum_{t \in \Ocb} \bar{h}_{t}s_{t}}{\sum_{t \in \Ocb} s_{t}} \right) \geq 
     \bar{h}_{y}- \frac{\sum_{t \in \Ocb} \bar{h}_{t}s_{t}}{\sum_{t \in \Ocb} s_{t}}  + \pi \geq 
{h}_{y}- \frac{\sum_{t \in \Ocb}{h}_{t}s_{t}}{\sum_{t \in \Ocb} s_{t}}
\end{equation}
which conclude (\ref{eq:mm1}). \\ 
\textbf{Case 2: } $\tf{\bar{W} - \Wm} \geq \epsilon \coloneqq \pi / (2M)$. In this case, for some $\delta = \delta(\epsilon) \geq 0$ and $\alpha \in \Ocb$, we have that 
\begin{equation}
    h_y - h_{\alpha} \leq 1 - 2\delta
\end{equation}
To proceed, suppose \textcolor{red}{$h_y - h_t \geq 1 - \delta $ for $t \in \Nc \text{ and } \Nc \subset \Ocb $} and $h_y - h_{t} < 1 - \delta$ for $t \in \Ocb - \Nc$. Then we have:
\begin{equation}
\begin{split}
     {h}_{y}- \frac{\sum_{t \in \Ocb} {h}_{t}s_{t}}{\sum_{t \in \Ocb} s_{t}} 
    &= \frac{\sum_{t \in \Ocb}(h_y - {h}_{t})s_{t}}{\sum_{t \in \Ocb} s_{t}}  \\   
    &\leq 
    \frac{\sum_{t \in \Nc} (h_y - h_{t}) s_{t}}{\sum_{t \in \Ocb} s_{t}}  + \frac{\sum_{t \in \Ocb - \Nc} (h_y - h_t) s_{t}}{\sum_{t \in \Ocb} s_{t}} \\ 
    & \textcolor{red}{<}
    1 - \delta + \frac{\sum_{t \in \Nc} (h_y - h_{t}) s_{t}}{\sum_{t \in \Ocb} s_{t}} \\ 
    &\leq 
    1 - \delta + 2 \max_{t \in [T]}\|h_t\| \frac{\sum_{t \in \Nc} s_{t}}{\sum_{t \in \Ocb} s_{t}} \\ 
\end{split}
\end{equation}
Note that 
\begin{equation}
   \frac{\sum_{t \in \Nc} s_{t}}{\sum_{t \in \Ocb} s_{t}} \leq \frac{\sum_{t \in \Nc} s_{t}}{s_{\alpha}} \leq T \frac{e^{\bar{R}(h_y + \delta - 1)}}{e^{\bar{R}(h_y + 2\delta - 1)}} = T \cdot e^{-\bar{R}\delta}\\ 
\end{equation}
where $s = \sft{\bar{R}\hb}, \bar{R} = \tf{\W} / \tf{\Wm}$. As a result
\begin{equation}
\begin{split}
{h}_{y}- \frac{\sum_{t \in \Ocb} {h}_{t}s_{t}}{\sum_{t \in \Ocb} s_{t}} 
     & \leq 1 - \delta + 2 \tf{\Wm}\cdot \|\x_{t}\xl^{\top}\|T e^{-\bar{R}\delta} \\ 
     & \leq 1 - \delta + 2\bar{M}Te^{-\bar{R}\delta} \\ 
    & \leq 1 + \pi' 
\end{split}
\end{equation}
where $\bar{M} = \tf{\Wm} \cdot \sup_{i,t} \|\x_{it}\xli^{\top} \|  $. Similar to Case 1, using the fact that $
\bar{h}_{y}- \frac{\sum_{t \in \Ocb} \bar{h}_{t}s_{t}}{\sum_{t \in \Ocb} s_{t}}  \geq 1$
and setting $\pi' < \pi$, we can then obtain (\ref{eq:mm1}) with 
\begin{equation}
    R_{\pi} = \delta^{-1}\tf{\Wm}\log(2\bar{M}T/\pi)   \text{ to ensure that } \pi' = \pi - \delta \leq \pi 
\end{equation}
\end{proof}
\subsubsection{Proof of Theorem \ref{thm:acyclic}}

\begin{proof}
    Given any $\epsilon \in (0,1 )$, let $\pi  = \epsilon / (1-\epsilon)$. Theorem \ref{thm:w} has shown that $\lim_{k \to \infty} \tf{W(k)} = \infty$. Hence, there exists some $k_0$ such that for $k \geq k_0$, it holds that $\tf{\W(k)} > R_{\epsilon} \vee 1/2 $ for some parameter $R_{\epsilon}$. Then using Lemma \ref{le:corr}, for $k \geq k_0$
    \begin{equation}
        \bigg \langle - \nabla \mathcal{L}(\W(k)), \frac{\Wm}{\tf{\Wm}} \bigg \rangle \geq (1 - \epsilon) \bigg \langle -\nabla \mathcal{L}(\W(k)), \frac{\W}{\tf{\W}} \bigg \rangle 
    \end{equation}
    Multiplying both sides by the stepsize $\eta$ and using (\ref{eq:wgd}), we get
    \begin{equation}
    \begin{split}
        \bigg \langle  \W(k+1) - \W(k), \frac{\Wm}{\tf{\Wm}} \bigg \rangle &\geq (1 - \epsilon) \bigg \langle \W(k+1) - \W(k), \frac{\W}{\tf{\W}} \bigg \rangle \\ 
        & = \frac{1- \epsilon}{2\tf{\W(k)}} \bigg(\tf{\W(k+1)}^2 - \tf{\W(k)}^2 - \tf{\W(k+1) - \W(k)}^2 \bigg) \\ 
        & \stackrel{(a)}\geq (1- \epsilon) \bigg(\frac{\tf{\W(k+1)}^2 - \tf{\W(k)}^2}{2\tf{\W(k)}} - \tf{\W(k+1) - \W(k)}^2 \bigg) \\ 
        & \stackrel{(b)}\geq (1- \epsilon) \bigg({\tf{\W(k+1)} - \tf{\W(k)}} - \tf{\W(k+1) - \W(k)}^2 \bigg) \\ 
        & \stackrel{(c)}\geq (1- \epsilon) \bigg({\tf{\W(k+1)} - \tf{\W(k)}} - 2\eta (\mathcal{L}(\W(k)) - \mathcal{L}(\W(k+1))) \bigg) \\ 
    \end{split}
    \end{equation}
    where (a) uses $\tf{\W(k)} \geq 1/2$, (b) derive from the fact that for any $x, y > 0, (x^2 - y^2)/(2y) - (x-y) \geq 0$ and (c) follows Lemma \ref{le:des}. \\
    Summing the above inequalities over $k \geq k_0$ gives 
    \begin{equation}
        \bigg \langle  \frac{\W(k)}{\tf{\W(k)}} , \frac{\Wm}{\tf{\Wm}} \bigg \rangle \geq 1 - \epsilon + \frac{C(\epsilon, \eta)}{\tf{\W(k)}} 
    \end{equation}
    for some finite constant $C(n, \eta) $ given as
    \begin{equation}
        C(\epsilon, \eta) = \big \langle {\W(k_0), \frac{\Wm}{\tf{\Wm}}}\big \rangle + 2\eta(1-\epsilon) (\mathcal{L}_{\bigstar} - \mathcal{L}(\W(k_0))) - (1-\epsilon)\tf{\W(k_0)}
    \end{equation}
    where $\mathcal{L}_{\bigstar} \leq \mathcal{L}(\W(k)) $ for all $k > 0$.\\ 
    Since $\| \W(k) \| \to \infty$, we eventually get 
    \begin{equation}
        \liminf_{k \to \infty} \bigg \langle  \frac{\W(k)}{\tf{\W(k)}} , \frac{\Wm}{\tf{\Wm}} \bigg \rangle \geq 1 - \epsilon
    \end{equation}
    Given that $\epsilon$ is arbitrary, we can consider the limit as $\epsilon$ approaches zero. Thus $\W(k) / \tf{\W(k)} \to \Wm / \tf{\Wm} $.
    \end{proof}
\subsection{Global Convergence: general data}
\subsubsection{Proof of Theorem \ref{thm graph bias}}
\redp{1. Whether we need zero initialization. 2. Whether we need Assumption \ref{assume realizable} and \ref{assume orth} for the Theorem. 3. Assumption \ref{assume relax} is used for regularization analysis of Theorem \ref{thm graph bias}}

Preliminaries:
From Assumption \ref{assume orth} and Lemma \ref{le:red2} we have 
    \begin{equation*}
        \Wm = \sum_{k=1}^K \Wm_k
    \end{equation*}
\subsection{Global Convergence: decomposition}
\subsubsection{Proof of Lemma \ref{lemma ortho}}
\begin{itemize}
    \item First we assume that $\Wf\subset \Scf$ is wrong and project $\Wf$ to the subspace $\Scf$: $\W_p = \prj_{\Scf}(\Wf) \neq \Wf$. Consider input $(\X, y) \in \bdata$ whose last token is $\xl = \eb_k$. 
    % \redp{TODO: Prove $\X \W_p \eb_k = \X \W \eb_k$ }
    To proceed, we focus on token $\x \in \X \text{ and } \x = \eb_j$ for some $j \in \Cck_i$. Based on Assumption \ref{assume orth}, we have
    \begin{equation}
    \begin{split}
        \eb_k^{\top}\eb_k = 1 &, \eb_\tau^{\top}\eb_k = 0 \\ 
        \x^{\top}\eb_j = 1 &, \x^{\top}\eb_t = 0 \\ 
    \end{split}
    \end{equation} 
    where $k \neq \tau, t \neq j, k, t \in [K]$. Recall the definition of $\Scf$ is the span of $(\eb_j-\bmu^{(k)}_i)\eb_k^\top \text{ for } j\in\Cck_i,i\in[N_k],k\in[K]$. As a result, we have 
    \begin{equation} \label{eq:equal}
        \x \W_p \xl = \x \Wf \xl
    \end{equation}
    Thus $\Wf \text{ and } \W_p$ achieve the same empirical risk over $\bdata$. At the same time, since $\Wf \neq \W_p$, $\tf{\Wf}^2 = \tf{\W_p}^2 + \tf{\Wf - \W_p}^2 > \tf{\W_p}^2 $, which leads to a contradiction that $\Wf$ is the min-norm solution. 
    \item To proceed, we assume $\Wm\perp \Scf$ is wrong and project $\Wm$ to the subspace $\Scf$: $\Wm_p = \prj_{\Scf}(\Wm) \neq \textbf{0}$. Recall in \eqref{graph svm}, we have 
    \begin{equation}
        (\eb_i - \eb_j)^{\top}\Wm\eb_k = 0 \text{ for all } i\asymp j \in \Gck \text{ and } k \in [K]
    \end{equation}
    From definition \ref{cyc sub}, for all $(\Xs, y) \in \bdata$ and all $i,j \in \Xs$, we have $i \asymp j$. Specifically they are all in the same SCC that contains $y$. Then we get:
    \begin{equation} 
        (\eb_i - \eb_j)^{\top} \Wm \eb_k = 0 \text{ for all } i, j \in \Xs \text{ and } (\Xs, y) \in \bdata
    \end{equation}
    From the definition of $\Scf$, we also have $\eb_j^{\top}\Wm\eb_k = \eb_j^{\top}\Wm_p \eb_k$ for any $j \in \Gck$
    which implies 
    \begin{equation}
        \x_i \Wm_p \xl = \x_j \Wm_p \xl \text{ for all } \x_i, \x_j \in \X \text{ and } \X \in \bdata
    \end{equation}
    As a result, we obtain a solution with the lower norm by subtracting $\Wf$ with $\Wm_p \neq \textbf{0}$ from while keeping the same risk as $\Wf$: $\tf{\Wf}^2 = \tf{\Wf - \Wm_p}^2 + \tf{\Wm_p}^2 > \tf{\Wf - \Wm_p}^2$, which leads to a contradiction with the assumption. 
    % \begin{equation}
    %     \X \Wf\xl = \X (\Wf - \Wm_p) \xl
    % \end{equation}
    % \redp{TODO: Prove $(\eb_i - \eb_j)^{\top} \Wm_p \eb_k = (\eb_i - \eb_j)^{\top} \Wm \eb_k$ }
\end{itemize}
% \redp{1. Prove by contradiction 2. Proof by contradiction by subtract Wfin with proj wmm(Wfin)}
\subsubsection{Decomposing gradient}
We project the gradient of $\Lc(\W)$ to the subspace $\Scf$ and $\Scf^{\perp}$ as the following:
\begin{equation}
\begin{split}
     \nabla \Lc(\W) 
     &= \prj_{\Scf}\nabla \Lc(\W) + \prj_{\Scf^{\perp}}\nabla \Lc(\W) \\ 
     &= \frac{1}{n}\sum_{i=1}^n \ell' \big(\bgam_i^{\top}\sft{\hb_i}\big)\big(\X_{\perp}^{\top} \sft{\X_{\perp}\W\xli}\bgam_i\xli^{\top} + \X_{\Scf}^{\top} \sft{\X_{\Scf}\W\xli}\bgam_i\xli^{\top} \big) \\
     &= \frac{1}{n}\sum_{i=1}^n \ell' \big(\bgam_i^{\top}\sft{\hb_i}\big)\big(\X_{\perp}^{\top} \sft{\X_{\perp}\prj_{\Scf^{\perp}}(\W)\xli} + \X_{\Scf}^{\top} \sft{\X_{\Scf}\prj_{\Scf}(\W)\xli} \big)\bgam_i\xli^{\top} \\ 
\end{split}
\end{equation}
where $\X_{\Scf} = \prj_{\Scf}\X, \X_{\perp} = \prj_{\Scf^\perp}\X $ 
\begin{lemma}
    $\X_{\Scf}$ only contains the edges inside the SCCs that contain the label while $\X_{\perp}$ contains the edges from the labels to nodes that is not in the same SCC as the corresponding label.
\end{lemma}
\subsubsection{Proof of Theorem \ref{thm: decompose}}
\redp{1. Prove correlation 2. Prove the norm goes to infinity.}
