# Supplementary material for: Mechanics of Next Token Prediction with Self-Attention
Source: arXiv:2403.08081 source file (2024-03-12)
Supplement: Supplementary file 2 [file automation.tex]

\begin{lemma}
    Assume the data sequence is generated from a discrete mapping from the vocabulary $\Eb$, i.e., $\X \coloneqq \Pb \Eb$ where $\Pb \in \R^{T \times K}$ is a universal mapping matrix. Define a \shaw{universal} dataset $\widetilde{\data} \coloneqq \{(\Xt_i, y_i)\}_{i=1}^n, \Xt = \Pb \Ebt = \Pb\Ib_K$ where the token embedding $\Ebt \coloneqq \Ib_K$ is the standard basis of $\R^K$. Set the SVM solutions of \eqref{graph svm} on the universal dataset and general dataset as $\tWm$ and $\Wm$ respectively. Assume $\widetilde{\data}$ and $\data$ share the same mapping matrix $\Pb$ and the token embedding of $\data$ satisfies $\text{rank}(\Eb) = K \leq d$, then we have:
    \begin{equation}
        \Wm = \Eb^{\dagger}\tWm(\Eb^{\dagger})^{\top}
    \end{equation}
    where $\Eb^{\dagger}$ is the pseudo-inverse of $\Eb$ satisfying $\Eb\Eb^{\dagger} = \Ib_K$. Or equivalently: $\tWm = \Eb\Wm\Eb^{\top}$
    % Define $\Lct(\Wt) \coloneqq \frac{1}{n}\sum_{i=1}^n \ell(\cb_{y_i}^{\top}\X^{\top}_i\mathbb{S}(\Pb_i\Wt\bar \pb_i )), \Lc(\W) \coloneqq \frac{1}{n}\sum_{i=1}^n \ell(\cb_{y_i}^{\top}\X^{\top}_i\mathbb{S}(\X_i\W\xli)).$ Suppose the gradient descent starts from $\Wt(0) \in \R^{K \times K} \text{ and } \W(0) = \Eb^{\dagger}\Wt(0)(\Eb^{\dagger})^{\top} \in \R^{d \times d}$ with step size $\eta$:
    % \begin{equation}
    %     \Wt(\tau+1) = \Wt(\tau) - \eta \nabla \Lct(\Wt(\tau)), \\ 
    %     \W(\tau+1) = \W(\tau) - \eta \nabla \Lc(\W(\tau)). 
    % \end{equation}
    % We have that $\W(\tau) = \Eb^{\dagger}\Wt(\tau)(\Eb^{\dagger})^{\top} $ for all $\tau \geq 0$. 
    % \shaw{Only for $\text{rank}(\Eb) = K \leq d$, otherwise $\Eb\Eb^{\dagger} \neq \Ib_{K}$}
\end{lemma}

\begin{proof}
When $\Eb\Eb^{\dagger} = \Ib_K$
\begin{equation}
    \eb_j = \Eb^{\top} \tilde{\eb}_j \leftrightarrow \tilde{\eb}_j = (\Eb^{\top})^{\dagger}\eb_j 
    \text{ for all } j \in [K] 
\end{equation}
Provided the SVM solution $\tWm$ on the universal dataset, for any $i, j$ induces an SVM constriant in \eqref{graph svm} by either $(i\asymp j) \in\Gck \text{ or } (i\Rightarrow j) \in\Gck$, we have:
\begin{equation}
    (\ebt_i - \ebt_j)^{\top}\tWm\ebt_k = (\eb_i - \eb_j)^{\top}\Eb^{\dagger}\tWm(\Eb^{\dagger})^{\top}\eb_k = (\eb_i - \eb_j)^{\top}\Wm\eb_k
\end{equation}
This implies that if $\tWm$ is the SVM solution on the universal dataset $\widetilde{\data}$, $\Wm = \Eb^{\dagger}\tWm(\Eb^{\dagger})^{\top}$ can also satisfy the same constraint on the general dataset $\data$ which shares the same discrete mapping with the universal dataset. 

\shaw{Next, we prove that $\Wm = \Eb^{\dagger}\tWm(\Eb^{\dagger})^{\top}$ is the minimal norm solution.} \textbf{However, we find that this may not be true for some examples.} Instead, when $\Eb\Eb^{\top} = \Eb \Eb^{\dagger} = \Ib_K$, we get $\Eb^{\dagger} = \Eb^{\top}(\Eb \Eb^{\top})^{-1} = \Eb^{\top}$, then for any $\W$, we have
\begin{equation}
    \tf{\Eb^{\dagger} \Wt (\Eb^{\dagger})^{\top}} = \tf{\Eb^{\top} \Wt \Eb} = \sqrt{\text{tr}(\Eb^{\top}\Wt^{\top}\Eb\Eb^{\top}\Wt\Eb)} = \sqrt{\text{tr}(\Wt^{\top}\Wt)} = \tf{\Wt}
\end{equation}
As a result, if $\tf{\tWm_{*}} \leq \tf{\tWm}$, we have:
\begin{equation}
    \tf{\Wm_*} = \tf{\Eb \tWm_* \Eb^{\top}}  = \tf{\tWm_{*}} \leq \tf{\tWm} = \tf{\Eb \tWm \Eb^{\top}} = \tf{\Wm}
\end{equation}
\end{proof}
