# Supplementary material for: Mechanics of Next Token Prediction with Self-Attention
Source: arXiv:2403.08081 source file (2024-03-12)
Supplement: Supplementary file 3 [file cvg_rate.tex]

\begin{lemma}[Smoothness-based GD bounds]\label{lemma: smooth} Suppose $\mathcal{L}$ is convex, and there exists $\beta \geq 0$, so that $1 - \eta_{\tau} \beta / 2 \geq 0 $ and assume for gradient descent $\W(\tau+1) = \W(\tau) - \eta_\tau \grad{\W(\tau)}$, we have:
\[
    \Lc(\W(\tau+1)) \leq \Lc(\W(\tau)) - \eta_{\tau} (1 - \frac{\eta_{\tau}\beta}{2}) \tf{\grad {\W(\tau)}}^2
\]
where $\eta_{\tau}$ is the step size at step $\tau$, then for any $\M \in \R^{d \times d}$, 
\[
    2 \sum_{j=0}^{\tau-1} \eta_{j} (\Lc(\W(j)) - \Lc(\M)) - \sum_{j=0}^{\tau-1} \frac{\eta_j}{1 - \eta_j \beta / 2}(\Lc(\W(j)) - \Lc(\W(j+1))) \\ \leq \tf{\W(0)- \M}^2 - \tf{\W(\tau) - \M}^2
\]
\end{lemma}
\begin{proof} The proof follows \cite{ji2019risk}. Set $r_\tau \coloneqq \eta_{\tau}(1 - \beta\eta_\tau/2)$
\begin{equation}
\begin{split}
    \tf{\W(\tau + 1) - \M}^2 
    & =  \tf{\W(\tau) - \M}^2 - 2\eta_\tau \langle \W(\tau) - \M, \nabla \Lc(\W(\tau)) \rangle + \eta_{\tau}^2 \tf{\grad{\W(\tau)}}^2 \\ 
    &\stackrel{(a)}{\leq}  \tf{\W(\tau) - \M}^2 - 2\eta_\tau \langle \W(\tau) - \M, \nabla \Lc(\W(\tau)) \rangle + \frac{\eta_{\tau}^2}{r_{\tau}} (\Lc(\W(\tau)) - \Lc(\W(\tau+1)))  \\ 
    & \stackrel{(b)}{\leq}  \tf{\W(\tau) - \M}^2 + 2\eta_{\tau}(\Lc(\M) - \Lc(\W(\tau))) + \frac{\eta_{\tau}^2}{r_{\tau}} (\Lc(\W(\tau)) - \Lc(\W(\tau+1)))  \\ 
\end{split}
\end{equation}
where (a) uses the condition that $\Lc(\W(\tau+1)) \leq \Lc(\W(\tau)) - \eta_{\tau} (1 - \frac{\eta_{\tau}\beta}{2}) \tf{\grad {\W(\tau)}}^2$. Note that from Lemma \ref{lemma des}, we can easily fulfill this condition by setting $\beta = L$ where $L$ is the Lipschitzness of $\grad{\W}$. And (b) comes from the convexity of $\Lc(\W)$. Summing the inequality over $j \in [\tau]$ and rearranging it gives the bound. 
\end{proof}

\begin{lemma}[Inserting a reference point]\label{lemma:ref} Suppose $\ell(u) = -\log(u)$. \shaw{Let the maximum of the token embedding to be $e_{max} \coloneqq \max_{k \in [K]} \|\eb_k\|$ and $\xi \coloneqq \min_{i} \min_{t \in \mathcal{R}_i, \tau \in \bar{\mathcal{R}}_i} (\x_{it} - \x_{i \tau})^TW^{mm}\xb_i / \tf{\Wm}$} Then for $\M \coloneq  W^{cyc} + \frac{\ln(\tau)}{\xi}\frac{\Wm}{\tf{\Wm}}$, we have:
    \begin{equation}
        \Lc(\M) \leq \inf_{\W} \Lc(\W) + \frac{T \cdot \exp({2\|W^{cyc}\|_F e_{max}^2})}{\tau}
    \end{equation}
Additionally, we have 
% $\tf{\M}^2 = \tf{\W^{cyc}}^2 + \ln(\tau)^2 * \tf{\Wm}^2 /\xi^2 $
$\tf{\M}^2 = \tf{\W^{cyc}}^2 + \ln(\tau)^2 /\xi^2 $
\end{lemma}
\begin{proofsk}
\shaw{We argue that the loss $\Lc(\M)$ can be upper bounded by the losses induced by correcting the probabilities inside the strongly connected components $\Lc_1$ and separating the tokens with different priorities $\Lc_2$ respectively using the concavity of $\log$ loss. For $\Lc_1$, we can prove that it is essentially the loss on the reduced dataset $\bdata$ and that the lower bound of the loss should be the same as the lower bound of the whole loss, i.e., $\inf_{\W} \Lc(\W) = \inf_{\W} \bar{\Lc}{(\W)}$. For the second part of the loss, we show that when $\tau \to \infty$, the loss will vanish eventually.} 
\end{proofsk}
\begin{proof}
For convenience, we set $\bWm = \Wm / \tf{\Wm}, b_{it} = \x_{it}^{\top}\W^{cyc} \xb_i, a_{it} = \x_{it}^{\top} \bWm \xb_i / \xi, a_{it'} = \x_{it'}^{\top} \bWm \xb_i / \xi$.  Based on \eqref{graph svm}, when $t_1, t_2 \in \mathcal{R}_i$, we have $a_{it_1 } = a_{it_2}$, then for any $t \in \mathcal{R}_i$, we set $a_{it} = \bar a_i$. Recap the dataset $\data=(\X_i,y_i)_{i=1}^n$ and index sets $\Oc_i,\Ocb_i,\Rc_i,\Rcb_i$, $i\in[n]$ from \eqref{def Oc Rc}, we can write $\Lc(\M)$ as:
\begin{equation}
\begin{split}
\mathcal{L}(\M) 
&= \frac{1}{n}\sum_{i=1}^n 
-\log (\frac{\sum_{t \in \mathcal{O}_i} e^{\x_{it}^{\top}\M\bar \x_i}}{\sum_{t' \in [T_i]} e^{\x_{it'}^{\top}\M\bar \x_i}}) \\ 
&= \frac{1}{n}\sum_{i=1}^n -\log (\frac{\sum_{t \in \mathcal{O}_i} e^{b_{it} + \ln(\tau) a_{it}} }{\sum_{t' \in [T_i]} e^{b_{it'} + \ln(\tau) a_{it'}}})
\\
&\stackrel{(a)}{=} \frac{1}{n}\sum_{i=1}^n -\log (\frac{\sum_{t \in \mathcal{O}_i} e^{b_{it} + \ln(\tau) \bar a_{i}} }{\sum_{t' \in \mathcal{R}_i} e^{b_{it'} + \ln(\tau) \bar a_i} + \sum_{t' \in \bar{\mathcal{R}_i}} e^{b_{it'} + \ln(\tau) a_{it'}}})
\\
& = \frac{1}{n}\sum_{i=1}^n -\log (\frac{\sum_{t \in \mathcal{O}_i} e^{b_{it}} }{\sum_{t' \in \mathcal{R}_i} e^{b_{it'}}  + e^{- \ln(\tau)\bar a_i}\sum_{t' \in \bar{\mathcal{R}}_i} e^{b_{it'} + \ln(\tau) a_{it'}}})
\\
& \stackrel{(b)}{\leq} \frac{1}{n}\sum_{i=1}^n \Big(
-\log (\frac{\sum_{t \in \mathcal{O}_i} e^{b_{it}} }{\sum_{t' \in \mathcal{R}_i} e^{b_{it'}}}) + \frac{\sum_{t' \in \bar{\mathcal{R}}_i} e^{b_{it'} + \ln(\tau) (a_{it'} - \bar a_i)}}{\sum_{t' \in \mathcal{R}_i} e^{b_{it'}}}\Big)
\\
&\leq \frac{1}{n}\sum_{i=1}^n -\log (\frac{\sum_{t \in \mathcal{O}_i} e^{b_{it}} }{\sum_{t' \in \mathcal{R}_i} e^{b_{it'}}}) + \frac{|\bar{\mathcal{R}}_i|e^{\max_{t' \in \bar{\mathcal{R}}_i}\big(b_{it'} + \ln(\tau) (a_{it'} - \bar a_i)\big)}}{\sum_{t' \in \mathcal{R}_i} e^{b_{it'}}} 
\end{split}
\end{equation}

where (a) comes from the fact that $a_{it} = \bar{a}_i$ for any $t \in \Rc_i$ and $\Oc_i \subseteq \Rc_i$ for any $i \in [n]$ and (b) follows the concavity of $\log(x)$ function, i.e., $\log(x + y) \leq \log(y) + \frac{x}{y} \text{ for any } x, y > 0$.
Note that from \eqref{graph svm}, we have $\xi > 0$, then for any $i \in [n]$,
\begin{equation}
\begin{split}
\max_{t' \in \bar{\mathcal{R}}_i} \big(b_{it'} + \ln(\tau) (a_{it'} - \bar a_i)\big)
& = \max_{t' \in \bar{\mathcal{R}}_i} b_{it'} + \max_{t' \in \bar{\mathcal{R}}_i} \ln(\tau) (a_{it'} - \bar a_i) \\
& = \max_{t' \in \bar{\mathcal{R}}_i}(\x_{it'}^{\top}\W^{cyc}\bar \x_i) - \ln(\tau) \min_{t \in \mathcal{R}_i, t' \in \bar {\mathcal{R}_i}} (\x_{it} - \x_{it'})^{\top}\bWm\bar \x_i / \xi \\
& \stackrel{(a)}{\leq} \tf{\W^{cyc}} e_{max}^2 - \ln(\tau) \min_{t \in \mathcal{R}_i, t' \in \bar {\mathcal{R}_i}} (\x_{it} - \x_{it'})^{\top}\bWm\bar \x_i / \xi \\
& \stackrel{(b)}{\leq} \tf{\W^{cyc}} e_{max}^2 - \ln(\tau) \\
\end{split} 
\end{equation}
where (a) comes from $|\x_{it'}^{\top}\W^{cyc}\bar \x_i| \leq \tf{\W^{cyc}} \|\bar x_i \|\|\x_{it'} \|$ and (b) follows the fact that for any $i \in [n]$, $\min_{t \in \mathcal{R}_i, \tau \in \bar{\mathcal{R}}_i} (\x_{it} - \x_{i \tau})^T\bWm\xb_i \geq \xi > 0$. As a result, we get:
\begin{equation}
\begin{split}
\Lc(\M) 
&\leq \frac{1}{n}\sum_{i=1}^n -\log (\frac{\sum_{t \in \mathcal{O}_i} e^{b_{it}} }{\sum_{t' \in \mathcal{R}_i} e^{b_{it'}}}) +  \frac{|\bar{\mathcal{R}}_i|e^{\tf{\W^{cyc}} e_{max}^2 - \ln(\tau)}}{\sum_{t' \in \mathcal{R}_i} e^{b_{it'}}} \\
&\leq  \frac{1}{n}\sum_{i=1}^n -\log (\frac{\sum_{t \in \mathcal{O}_i} e^{b_{it}} }{\sum_{t' \in \mathcal{R}_i} e^{b_{it'}}}) + \frac{|\bar{\mathcal{R}}_i|e^{\tf{\W^{cyc}} e_{max}^2}}{\tau * e^{-\tf{\W^{cyc}} e_{max}^2}} \\ 
&\stackrel{(a)}{=} \inf_{\W} \Lc(\W) + \frac{|\bar{\mathcal{R}}_i|\exp({2 \tf{\W^{cyc}} e_{max}^2})}{\tau} \\ 
&{=} \inf_{\W} \Lc(\W) + \frac{T\cdot \exp({2 \tf{\W^{cyc}} e_{max}^2})}{\tau} 
\end{split} 
\end{equation}
\shaw{where (a) comes from the Definition of $\W^{cyc}$ in Definition \ref{def finite correct}}. Lastly, since $\W^{cyc} \perp \Wm$ from Lemma \ref{lemma ortho}, we have:
\begin{equation}
\tf{\M}^2 = \tf{\W^{cyc}}^2 + \ln(\tau)^2 /\xi^2 
\end{equation}
\end{proof}

\begin{theorem}
    Suppose $\ell(u) = -log(u)$, given step size $\eta_j \leq 1/L$, where $L$ is defined in \eqref{lip term}, and $\W(0) = 0$, for any $\tau \geq 1$, we have:
    \begin{equation}
        \Lc(\W(\tau)) - \inf_{\W} \Lc(\W) \leq \frac{T \cdot \exp({2\|W^{cyc}\|_F e_{max}^2})}{\tau} + \frac{\tf{\W^{cyc}}^2 + \ln(\tau)^2 / \xi^2}{2 \sum_{j=0}^{\tau-1} \eta_{j}} 
    \end{equation}
    
    where $e_{max} \text{ and } \xi$ are defined in Lemma \ref{lemma:ref}.
    
    Furthermore, we have:
    \begin{equation}
        \Lc(\W(\tau)) - \inf_{\W} \Lc(\W) \leq \mathcal{O}(\frac{T}{\tau} + \frac{\ln(\tau)^2}{\sum_{j < \tau}\eta_j}) = \begin{cases}
            \mathcal{O}(\ln(\tau)^2/\tau) & \eta_j = \Omega(1), \\ 
            \mathcal{O}(\ln(\tau)^2/\sqrt{\tau}) & \eta_j = \Omega(1/\sqrt{j+1}), \\      
        \end{cases}
    \end{equation}
    % where \shaw{$\mathcal{O}$ is the }
\end{theorem}
\begin{proof}
    From Lemma \ref{lemma des}, for any $\tau \geq 0$, we have:
    \begin{equation}\label{eq:decreasing}
    \Lc(\W(\tau+1)) \leq \Lc(\W(\tau)) - \eta_{\tau} (1 - \frac{\eta_{\tau}L}{2}) \tf{\grad {\W(\tau)}}^2 \leq \Lc(\W(\tau))
    \end{equation}
    Then using Lemma \ref{lemma: smooth} when $\W(0) = 0 \text{ and } \eta_j L \leq 1$:
    \begin{equation}
    \begin{split}
     2 \big(\sum_{j=0}^{\tau-1} \eta_{j}\big)(\Lc(\W(\tau)) - \Lc(\M)) 
    & \stackrel{(a)}{\leq} 2 \sum_{j=0}^{\tau-1} \eta_{j} (\Lc(\W(j)) - \Lc(\M)) + 2 \sum_{j=0}^{\tau-1} \eta_{j} (\Lc(\W(j+1)) - \Lc(\W(j)) \\ 
    & {\leq} 2 \sum_{j=0}^{\tau-1} \eta_{j} (\Lc(\W(j)) - \Lc(\M)) - \sum_{j=0}^{\tau-1} \frac{\eta_j}{1 - \eta_j L / 2}(\Lc(\W(j)) - \Lc(\W(j+1)))  \\ 
    &\stackrel{(b)}{\leq} \tf{\M}^2 - \tf{\W(\tau) - \M}^2 \\ 
    & \leq \tf{\M}^2 \\ 
    \end{split}
    \end{equation}
    where (a) comes from $\Lc(\W(\tau+1)) \leq \Lc(\W(\tau))$ in \eqref{eq:decreasing} and (b) comes from Lemma \ref{lemma: smooth}. Combining Lemma \ref{lemma:ref} with the inequality above, we get:
    \begin{equation}
    \begin{split}
        \Lc(\W(\tau)) 
        & \leq \Lc(\M) + \frac{\tf{\M}^2}{2 \sum_{j=0}^{\tau-1} \eta_{j}}    \\ 
        & \leq \inf_{\W} \Lc(\W)+ \frac{T \cdot \exp({2\|W^{cyc}\|_F e_{max}^2})}{\tau} + \frac{\tf{\W^{cyc}}^2 + \ln(\tau)^2 /\xi^2}{2 \sum_{j=0}^{\tau-1} \eta_{j}}    \\ 
    \end{split}
    \end{equation}
    From Lemma \ref{lemma finite wfin}, $\W^{cyc}$ is finite. 
    % Besides, \shaw{$\tf{\Wm} / \xi$ is also finite according to the definition of $\xi, \frac{\tf{\Wm}}{\xi} \leq $}. 
    \shaw{Thus, we get: (Do we need to take $\xi \coloneqq \min_{i} \min_{t \in \mathcal{R}_i, \tau \in \bar{\mathcal{R}}_i} (\x_{it} - \x_{i \tau})^TW^{mm}\xb_i / \tf{\Wm}$ into consideration?)}
    \begin{equation}
            \Lc(\W(\tau)) - \inf_{\W} \Lc(\W) \leq \mathcal{O}(\frac{T}{\tau} + \frac{\ln(\tau)^2}{\sum_{j < \tau}\eta_j}) = \begin{cases}
            \mathcal{O}(\ln(\tau)^2/\tau) & \eta_j = \Omega(1), \\ 
            \mathcal{O}(\ln(\tau)^2/\sqrt{\tau}) & \eta_j = \Omega(1/\sqrt{j+1}), \\      
        \end{cases}
    \end{equation}
\end{proof}
\begin{lemma}
    Prove that for any $\tau \geq 0$, there exists a constant $C > 0$, s.t. 
    \begin{align*}
    { \mathcal{L}(\Pi_{\perp} W_\tau)} \geq C\cdot  \frac{\|\Pi_{\perp}\mathcal{L}(W_\tau)\|_F}{2|e_{max}|^2}
    \end{align*}
    where $e_{max} = \max_{k \in [K]}\|e_k\|$.
\end{lemma}
\begin{proof}
Let $s_{i} = \mathbb{S}(X_iW_{\tau}\bar x_i), s_{i}^{\perp} = \mathbb{S}(X_i\Pi_{S_{cyc}^{\perp}}W_{\tau}\bar x_i)$. Lemma~\ref{lemma ortho} reveals that for any $t \in \Rc_i$, $x_{it}^{\top}\Pi_{S_{cyc}^{\perp}}W\bar x_i  = \Gamma$. As a result,
\begin{equation}
    s_{it}^{\perp}  = \frac{\exp(x_{it}^{\top}\Pi_{S_{cyc}^{\perp}}W\bar x_i)}{\sum_{t'} \exp(x_{it'}^{\top}\Pi_{S_{cyc}^{\perp}}W\bar x_i)} = \frac{\Gamma}{|\mathcal{R}_i|\Gamma +\sum_{t' \in \bar{\mathcal{R}}_i} \exp(x_{it'}^{\top}\Pi_{S_{cyc}^{\perp}}W\bar x_i) } \leq \frac{1}{|\mathcal{R}_i|}
\end{equation}
\begin{equation}
\begin{split}
\mathcal{L}(\Pi_{\perp} W_\tau) - \frac{C}{2 |e_{max}|^2 } \cdot \|\Pi_{\perp}\mathcal{L}(W_\tau)\|_F 
&=  \frac{1}{n}\sum_{i=1}^n \left(-\log\Big(\sum_{t\in\mathcal{O}_i}s_{it}^{\perp} \Big) - \frac{C}{2 |e_{max}|^2 }\| \sum_{t \in \bar {\mathcal{R}}_i}s_{it}(x_{it} - e_{y_i}) \bar x_i^{\top}\|_F\right) \\ 
&\stackrel{(a)}\geq  \frac{1}{n}\sum_{i=1}^n \left(-\log\Big(\sum_{t\in\mathcal{O}_i}s_{it}^{\perp} \Big) - C \cdot  \sum_{t \in \bar {\mathcal{R}}_i}s_{it} \right) \\
&\geq  \frac{1}{n}\sum_{i=1}^n C\left( \sum_{t \in \mathcal{R}_i}s_{it}-\frac{1}{C}\log\Big(\sum_{t\in\mathcal{O}_i}s_{it}^{\perp} \Big) - 1 \right) \\
&\stackrel{(b)}\geq \frac{1}{n}\sum_{i=1}^n C\left( \sum_{t \in \mathcal{R}_i}s_{it} - \frac{1}{C}\log\Big(\frac{|\mathcal{O}_i|}{|\mathcal{R}_i|} \Big) - 1\right) \\
&\geq \frac{1}{n}\sum_{i=1}^n C\left( \frac{|\mathcal{O}_i|}{T} - \frac{1}{C}\log\Big(\frac{|\mathcal{O}_i|}{|\mathcal{R}_i|} \Big) - 1\right) \\
\end{split}
\end{equation}
where (a) comes from the Cauchy-Schwarz inequality and (b) comes from $s_{it}^{\perp} \leq \frac{1}{|\Rc_i|} \text{ for } t \in \Rc_i$ derived above. \yl{The proof is problematic when $|\Oc_i|$ and $|\Rc_i|$ are equal.}
\end{proof}
% \begin{lemma}[smoothness estimates]
%     Suppose $\Lc(W)$ is convex, and $\hat \eta_{\tau} = \eta_{\tau}\Lc(\W(\tau)) \leq 1 $ \shaw{(need a upper bound of the loss)}. Then 
%     \begin{equation}
%         \Lc(\W(\tau+1)) \leq \Lc(\W(\tau)) - \eta_\tau(1 - \frac{\eta_\tau \Lc(\W(\tau))}{2})\tf{\grad{\W(\tau)}}^2 = \Lc(\W(\tau)(1 - \hat \eta_{\tau}(1 - \hat \eta_\tau / 2)\gamma_\tau^2) 
%     \end{equation}
%     and thus 
%     \begin{equation}
%         \Lc(\W(\tau)) \leq \Lc(\W(0)) \prod_{j < \tau}(1 - \hat \eta_{j}(1 - \hat \eta_j / 2)\gamma_j^2)
%     \end{equation}
%     Moreover, $\tf{\W(\tau)} \leq \sum_{j < \tau}\hat \eta_j \gamma_j$
% \end{lemma}
% \begin{proof}
%     From Lemma \ref{lemma des}, we have
%     \begin{equation}
%         \Lc(\W(\tau+1)) = \Lc (\W(\tau)) - \eta\left(1 -\frac{L \eta}{2}\right)  \tf{\nabla \Lc(\W(\tau))}^2 
%     \end{equation}
% \end{proof}
