# Supplementary material for: Mechanics of Next Token Prediction with Self-Attention
Source: arXiv:2403.08081 source file (2024-03-12)
Supplement: Supplementary file 4 [file gradient.tex]

\section{Global convergence of $\bf{W}^{mm}$}
% \subsection{Local optimal direction}
% \begin{definition}[Support indices and locally optimal tokens] \label{define local}
% Fix token indices $\bal = (\alpha_i)_{i=1}^n$. Solve \eqref{acyc svm}
% with $?$ replaced with $\bal = (\alpha_i)_{i=1}^n$ to obtain $\Wm_{\alpha}$. Consider the set $\Tc_i \subset [T]$ such that 
 
%  \end{definition}

\subsection{Connection between gradient descent and regularization path}
\begin{lemma}
    Suppose Assumption \ref{assume loss} and \ref{assume iden} hold and the loss function is $\ell(\cdot) = -\log(\cdot)$. If the step size $\eta \leq 1/L$, where $L$ is the smoothness defined in Lemma \ref{le:loss}. Then for any $\W \in \R^{d \times d}$, 
    \begin{equation} \label{eq:cvxbd}
        \tf{\W(\tau+1) - \W}^2 \leq \tf{\W(\tau) - \W}^2 + 2 \eta (\Lc(\W) - \Lc(\W(\tau+1)))
    \end{equation}
    This indicates $\tf{\W(\tau+1) - \W} \leq \tf{\W(\tau) - \W}$ if $\Lc(\W) \leq \Lc(\W(\tau+1))$. Consequently, 
    \begin{equation}
        \lim_{\tau \to \infty} \Lc(\W(\tau)) = \inf_{\W \in \R^{d \times d}} \Lc(\W)
    \end{equation}
    which implies $\lim_{\tau \to \infty}\tf{\W(\tau)} = \infty$ if the infimum of $\Lc$ is not attained. 
\end{lemma}
\begin{proof} \redp{This proof is adapted from \cite{ji2020gradient}}
When Assumption \ref{assume iden} holds and $\ell(\cdot) = -\log(\cdot)$, Lemma \ref{lemma cvx} shows that $\Lc(W)$ is convex. Moreover, under Lemma \ref{le:des} and $\eta \leq 1/L$, we have 
\begin{equation}
     \Lc(\W(\tau+1)) - \Lc(\W(\tau)) \leq -\frac{\eta}{2} \tf{\nabla \Lc(\W(\tau))}^2
\end{equation}
As a result, for any $\W \in \R^{d \times d}$ we get
    \begin{equation} \label{eq:cvxbd}
    \begin{split}
        \tf{\W(\tau+1) - \W}^2 
        &= \tf{\W(\tau) - \W}^2 - 2\eta\langle {\grad{\W(\tau)}, \W(\tau) - \W}\rangle + \eta^2 \tf{\grad{\W(\tau)}}^2 \\ 
        &= \tf{\W(\tau) - \W}^2 + 2\eta\langle {\grad{\W(\tau)}, \W - \W(\tau)}\rangle + \eta^2 \tf{\grad{\W(\tau)}}^2 \\ 
        &\stackrel{(a)}{\leq} \tf{\W(\tau) - \W}^2 + 2\eta{(\Lc(\W) - \Lc(\W(\tau)))} + \eta^2 \tf{\grad{\W(\tau)}}^2 \\
        &\stackrel{(b)}{\leq} \tf{\W(\tau) - \W}^2 + 2\eta{(\Lc(\W) - \Lc(\W(\tau)))} + 2\eta(\Lc(\W(\tau)) - \Lc(\W(\tau+1)))  \\
        &= \tf{\W(\tau) - \W}^2 + 2\eta(\Lc(\W) - \Lc(\W(\tau+1)))  \\
    \end{split}
    \end{equation}
    where (a) comes from the convexity of $\Lc(\W)$ and (b) comes from Lemma \ref{le:des}. To proceed, since $\Lc(W_{\tau})$ is nonincreasing and bounded from below, $\lim_{\tau \to \infty}\Lc(\W(\tau))$ exists. Suppose $\lim_{\tau \to \infty}{\Lc(\W(\tau))} > \inf_{\W \in \R{d \times d}}\Lc(\W)$. Then there exists $\epsilon > 0, \Wb \in \R^{d \times d}$ such that $\Lc(\Wb) < \lim_{\tau \to \infty}\Lc(\W(\tau)) - \epsilon$. Then following \eqref{eq:cvxbd}, we have $\tf{\W(\tau+1) - \Wb}^2 \leq \tf{\W(\tau) - \Wb}^2 - 2\eta \epsilon$ for any $\tau$, which leads to  $\tf{\W(\tau+1) - \Wb}^2 \leq \tf{\W_{0} - \Wb}^2 - 2\eta \epsilon \tau \to -\infty$ when $\tau$ goes to $\infty$, which is a contradiction. This concludes the lemma. 
\end{proof}
\begin{theorem}
    Consider the gradient descent and regularization path algorithms given in \ref{algo gd} and \ref{algo rp}. Suppose Assumption \ref{assume loss} holds, and $\ell(\cdot) = -\log(\cdot)$, and step size satisfies $\eta \leq 1/L \wedge 1/(2\Lc(\W_0))$. If $\lim_{\tau \to \infty}\W(\tau) / \tf{\W(\tau)} = \Wb$ for some matrix with $\tf{\Wb} = 1$, then we also have $\lim_{B \to \infty}\W_B / B = \Wb$ 
\end{theorem}
\begin{proofsk}
    
\end{proofsk}
\begin{proof}
    \redp{The proof follows \cite{}. COLT-2020-Ji}. First, we show that for any $\epsilon > 0$, there exists $B_1(\epsilon) > 0$, such that for any $\W(\tau)$ with $\W(\tau) > B_1(\epsilon)$, it holds that $\tf{\W(\tau) / \tf{\W(\tau)} - \Wb} < \epsilon$. Then if $\lim_{\tau \to \infty}\W(\tau) / \tf{\W(\tau)} = \Wb$, given any $\epsilon$, there exists $\tau_1$ such that $\tf{\W(\tau) / \tf{\W(\tau)} - \Wb} < \epsilon$ for $\tau > \tau_1$. It is sufficient to set $B_1(\epsilon) = \max_{\tau \in [\tau_1]} \tf{\W(\tau)} + 1$.\\
    Next we show that $\lim_{B \to \infty}\langle{\W_B, \Wb}\rangle \to \infty$. Suppose it is not true, then there exists a constant $C > 0$, such that there exists an arbitrarily large $B$ with $\langle{\W_B, \Wb} \rangle < C$. Choose $B_2$ such that 
    \begin{equation}
        B_2 > \max \{ 5(\tf{\W_0} + C + 1), B_1\left(\frac{1}{4}\right) + 1\}, \text{ and } \langle{\W_{B_2}, \Wb}\rangle < C
    \end{equation}
    Let $\tau_2$ denote the first step such that $\tf{\W_{\tau_2}} > B_2 - 1$. Since $B_2 - 1 > \tf{\W_0}$, we have $\tau_2 > 0$. Then if $\eta \leq 1/L \wedge 1/(2\Lc(\W_0))$, we have
    \begin{equation}\label{eq:diffw}
    \begin{split}
        \tf{\W_{\tau_2} - \W_{\tau_2 - 1}} = \eta \tf{\grad{\W_{\tau_2 - 1}}} &= \sqrt{\eta^2 \tf{\grad{\W_{\tau_2 - 1}}}^2} \\ 
                                & \stackrel{(a)}{\leq} \sqrt{2 \eta (\Lc(\W_{\tau_2 - 1}) - \Lc(\W_{\tau_2}))} \\ 
                                % & \stackrel{(b)}{\leq} \sqrt{2 \eta \Lc(\W_0))} \stackrel{(c)}{\leq} 1 
    \end{split}
    \end{equation}
    where (a) comes from Lemma \ref{le:des}. To proceed, we show that $\Lc(W_{\tau}) > 0$ for any $\tau$. When $\ell(\cdot) = -\log(\cdot)$ and Assumption \ref{assume iden} holds, the loss function is
    \begin{equation}
        \Lc(\W)=\frac{1}{n}\sum_{i=1}^n -\log(\cb_{y_i}^\top\X_i^\top \sft{\X_i\W\xli}) 
        % = \frac{1}{n}\sum_{i=1}^n -\log \bigg( \frac{e^{v_{iy}}} {\sum_{t \in [T_i]} e^{v_{it}}} \bigg)
    \end{equation}
    % where $v_{iy} = \eb_{y_i}^{\top}\W\xli, v_{it} = \x_{it}^{\top}\W\xli$
    If the input to $\ell(\cdot)$ is bounded in $(0, 1)$, $\Lc(W)$ is nonincreasing and bounded below by zero. This implies
    \begin{equation} \label{eq:diffloss}
        \Lc(\W_{\tau_2 - 1}) - \Lc(\W_{\tau_2}) \leq \Lc(\W_{\tau_2 - 1}) \leq \Lc(\W_0)
    \end{equation}
    Substituting \eqref{eq:diffloss} into \eqref{eq:diffw}, we get:
    \begin{equation}
        \begin{split}
              \tf{\W_{\tau_2} - \W_{\tau_2 - 1}} 
              &{\leq} \sqrt{2 \eta (\Lc(\W_{\tau_2 - 1}) - \Lc(\W_{\tau_2}))} \\ 
            & {\leq} \sqrt{2 \eta \Lc(\W_0)} \stackrel{(a)}{\leq} 1 
        \end{split}
    \end{equation}
    where (a) comes from $\eta \leq 1/(2\Lc(\W_0))$. Therefore from the definition of $\tau_2$, 
    \begin{equation} \label{eq:B2}
        \tf{\W_{\tau_2}} \leq \tf{\W_{\tau_2 - 1}} + \tf{\W_{\tau_2} - \W_{\tau_2 - 1}} \leq B_2 - 1 + 1 = B_2
    \end{equation}
    By the definition of $\tau_2$ and $\W_{B_2}$, we have $\Lc(\W_{B_2}) \leq \Lc(\W(\tau))$ for any $\tau \leq \tau_2$. On the one hand, using \eqref{eq:cvxbd}, we get 
    \begin{equation}\label{eq:wdiff1}
        \tf{\W_{\tau_2} - \W_{B_2}} \leq \tf{\W_0 - \W_{B_2}}  \stackrel{(a)}{\leq} \tf{\W_0} + \tf{\W_{B_2}} = \tf{\W_0} + B_2
    \end{equation}
    where (a) comes from the triangle inequality. On the other hand, 
    \begin{equation}
    \begin{split}
        \tf{\W_{\tau_2} - \W_{B_2}} ^2 
        &= \tf{\W_{\tau_2}}^2 + B_2^2 - 2 \langle \W_{\tau_2}, \W_{B_2} \rangle \\ 
        &= \tf{\W_{\tau_2}}^2 + B_2^2 - 2 \tf{\W_{\tau_2}}\left\langle \frac{\W_{\tau_2}}{\tf{\W_{\tau_2}}}, \W_{B_2}\right \rangle \\ 
        &> (B_2 - 1)^2 + B_2^2 - 2\tf{\W_{\tau_2}}\left\langle\frac{\W_{\tau_2}}{\tf{\W_{\tau_2}}}, \W_{B_2}\right \rangle \\ 
    \end{split}
    \end{equation}
    By the definition of $\tau_2 \text{ and } B_2$, we have 
    \begin{equation}
        \tf{\W_{\tau_2}} > B_2 -1 > B_1 \left(\frac{1}{4}\right)
    \end{equation}
    which implies $\tf{\W_{\tau_2}/\tf{\W_{\tau_2}} - \Wb} \leq 1/4$. As a result, 
    \begin{equation}
        \left\langle \frac{\W_{\tau_2}}{\tf{\W_{\tau_2}}}, \W_{B_2} \right\rangle < \langle \Wb, \W_{B_2} \rangle + \frac{1}{4} B_2 < C + \frac{1}{4} B_2
    \end{equation}
    which leads to
    \begin{equation}
    \begin{split} \label{eq:wdiff2}
        \tf{\W_{\tau_2} - \W_{B_2}} ^2 
        &> (B_2 - 1)^2 + B_2^2 - 2\tf{\W_{\tau_2}}\left\langle\frac{\W_{\tau_2}}{\tf{\W_{\tau_2}}}, \W_{B_2}\right \rangle \\ 
        &> (B_2 - 1)^2 + B_2^2 - 2\tf{\W_{\tau_2}}(C + \frac{1}{4}B_2) \\ 
        &\geq (B_2 - 1)^2 + B_2^2 - 2B_2(C + \frac{1}{4}B_2) > \frac{3}{2}B_2^2 -2CB_2 - 2B_2\\ 
    \end{split}
    \end{equation}
    Combining \eqref{eq:wdiff1} with \eqref{eq:wdiff2} yields
    \begin{equation}
        \frac{3}{2}B_2^2 -2CB_2 - 2B_2 < \tf{\W_0}^2 + 2 \tf{\W_0} {B_2} + B_2^2
    \end{equation}
    which implies 
    \begin{equation}
        B_2 < 4(\tf{\W_0} + C + 1) + \frac{2\tf{\W_0}^2}{B_2} \stackrel{(a)}{<} 4(\tf{\W_0} + C + 1) + \tf{\W_0} < 5(\tf{\W_0} + C + 1)
    \end{equation}
    where (a) comes from $B_2 > 5(\tf{\W_0} + C+ 1) > 2\tf{\W_0}$. This leads to a contradiction.\\
    For the next step, we prove that $\lim_{B \to \infty} \W_{B} / B = \Wb$. Suppose the claim is not true, then there exists $\delta > 0$, such that there is an arbitrarily large $B$ with $\tf{\W_B/B - \Wb} > \delta$. Choosing $B_4$ such that 
    \begin{equation}
        \tf{\frac{\W_{B_4}}{B_4} - \Wb} > \delta, \text{ and } \langle \W_{B_4}, \Wb \rangle > B_1\left(\frac{\delta^3}{32}\right) + \tf{\W(0)} + 1, \text{ and }B_4 > \frac{32}{\delta^3}
    \end{equation}
    Let $B_3 \coloneqq \langle \W_{B_4}, \Wb \rangle, \bar{B}_3 \coloneqq \frac{B_3}{B_4} = \langle \frac{\W_{B_4}}{B_4}, \Wb \rangle$. We have
    \begin{equation}
    \begin{split}
        \tf{\W_{B_4} - B_4\Wb} - \tf{\W_{B_4} - B_3\Wb} &=  \sqrt{B_4^2(1 -2 \langle{\frac{W_{B_4}}{B_4}, \Wb \rangle} + \Wb^2)} - \sqrt{B_4^2(1 -2 \langle{\frac{W_{B_4}}{B_4}, \frac{B_3}{B_4} \Wb \rangle} + (\frac{B_3}{B_4})^2 \Wb^2) } \\ 
        &= B_4 (\sqrt{2 - 2\bar{B}_3} - \sqrt{1 - \bar{B}_3^2})
    \end{split}
    \end{equation}
    Recall that $\tf{\frac{\W_{B_4}}{B_4} - \Wb} = \sqrt{2 - 2\bar{B}_3} > \delta$, then $\bar{B}_3 < 1 - \frac{1}{2}\delta^2$. Since $\bar{B}_3 \geq -1$, we have $\delta^2 < 4$. As a result, we get
    \begin{equation}\label{eq:diff3}
    \begin{split}
        \tf{\W_{B_4} - B_4\Wb} - \tf{\W_{B_4} - B_3\Wb} 
        &= B_4 (\sqrt{2 - 2\bar{B}_3} - \sqrt{1 - \bar{B}_3^2}) \\
        &\stackrel{(a)} > B_4 (\delta - \delta \sqrt{1 - \frac{1}{4}\delta^2 }) \\ 
        &> B_4 (\delta - \delta \sqrt{1 - \frac{1}{4}\delta^2 + \frac{1}{64}\delta^4}) \\ 
        &> B_4 (\delta - \delta |1 - \frac{1}{8}\delta^2|) > \frac{B_4 \delta^3}{8}\\ 
    \end{split}
    \end{equation}
    where (a) comes from the fact that $f(\bar{B}_3) = \sqrt{2 - 2\bar{B}_3} - \sqrt{1 - \bar{B}_3^2}$ is decreasing. 
    Similar to $B_2$, let $\tau_3$ denote the first step such that $\tf{\W(\tau_3)} > B_3 - 1$. Since $B_3 -1 > \tf{\W(0)}$, we have $\tau_3 > 0$, and we can show that $\W(\tau_3) \leq B_3$ following \eqref{eq:B2}. Since $B_3 - 1 > B_1(\delta^3/32)$, we have $\tf{\W(\tau_3) / \tf{\W(\tau_3)} - \Wb} < \delta^3 / 32$. As a result,
    \begin{equation}
    \begin{split}
        \tf{\W(\tau_3) - B_3\Wb} &\leq \tf{\W(\tau_3) - \tf{\W(\tau_3)}\Wb} + \tf{\tf{\W(\tau_3)}\Wb - B_3\Wb} \\
        &\leq \frac{\tf{\W(\tau_3)} \delta^3}{32} + 1 \leq  \frac{B_3 \delta^3}{32} + 1 \leq \frac{B_4 \delta^3}{32} + 1
    \end{split}
    \end{equation}
    Similarly, let let $\tau_4$ denote the first step such that $\tf{\W_{\tau_4}} > B_4 - 1$, we can show that $\tf{\W_{\tau_4}} \leq B_4$, and that
    \begin{equation}\label{eq:diff4}
        \tf{\W(\tau_4) - B_4\Wb} \leq \frac{B_4 \delta^3}{32} + 1
    \end{equation}
    Combining \eqref{eq:diff3} with \eqref{eq:diff4} gives
    \begin{equation}\label{eq:contrabd}
    \begin{split}
        & \tf{\W_{B_4} - \W(\tau_4)} - \tf{\W_{B_4} - \W(\tau_3)} \\ 
        &\geq  \tf{\W_{B_4} - B_4\Wb} - \tf{\W_{B_4} - B_3\Wb} - \tf{\W(\tau_4) - B_4\Wb} - \tf{\W(\tau_3) - B_3\Wb}  \\ 
        &\geq \frac{B_4 \delta^3}{8} - \frac{B_4 \delta^3}{32} - 1 - \frac{B_4 \delta^3}{32} - 1 \\ 
        &= \frac{B_4 \delta^3}{16} - 2 > 0
    \end{split}
    \end{equation}
    At the same time, 
    \begin{equation}
        B_4 - B_3 = \tf{{B_4}\Wb - B_3\Wb} \geq \tf{\W_{B_4} - B_4\Wb} - \tf{\W_{B_4} - B_3\Wb} >\frac{B_4 \delta^3}{8} > 4 
    \end{equation}
    Thus $\tau_4 > \tau_3$. Since $\tf{\W(\tau_4)} \leq B_4$, by the definition of $\tau_4$ and $\W_{B_4}$, we have $\Lc(\W_{B_4}) \leq \Lc(\W(\tau))$ for any $\tau \leq \tau_4$. Since $\tau_3 < \tau_4$, we have 
    $\tf{\W_{B_4} - \W(\tau_4)} \leq \tf{\W_{B_4} - \W(\tau_3)}$ from \eqref{eq:cvxbd}, which contradicts \eqref{eq:contrabd}. This concludes the proof. 
\end{proof}
\subsection{Divergence of ${\tf{{\bf{W}}(k)}}$}
\begin{lemma}[Descent Lemma] \label{le:des} Under Assumption \ref{assume loss}, if {$\eta \leq 1 / L$} where $L$ is the smoothness of $\Lc(\W)$ following Lemma~\ref{le:loss}, then for any initialization $\W(0)$, Algorithm \ref{algo gd} satisfies: 
\begin{equation}
     \Lc(\W(\tau+1)) - \Lc(\W(\tau)) \leq -\frac{\eta}{2} \tf{\nabla \Lc(\W(\tau))}^2
\end{equation}
for all $\tau \geq 0$. Additionally, it holds that $\sum_{\tau=0}^{\infty} \tf {\nabla \Lc(\W(\tau))}^2 < \infty$, and $\lim_{\tau \to \infty} \tf{\nabla \Lc(\W(\tau))}^2 = 0$
\end{lemma}
    \begin{proof}
From \eqref{algo gd}, we have that $\W(\tau+1)=\W(\tau)-\eta\nabla\Lc(\W(\tau))$. Since $\mathcal{L}(\W)$ is $L$-smooth following Lemma~\ref{le:loss}, we get
    \begin{equation}
    \begin{split}
        \Lc(\W(\tau+1)) 
        & \leq \Lc(\W(\tau)) + \langle {\nabla \Lc(\W(\tau)), \W(\tau+1) - \W(\tau) }\rangle + \frac{L}{2}\tf{\W(\tau+1) - \W(\tau)}^2 \\ 
        & = \Lc (\W(\tau)) - \eta\cdot \tf{\nabla \Lc(\W(\tau))}^2 + \frac{L \eta^2}{2}\tf{\nabla \Lc(\W(\tau))}^2 \\ 
        & = \Lc (\W(\tau)) - \eta(1 -\frac{L \eta}{2})  \tf{\nabla \Lc(\W(\tau))}^2 \\ 
        & \leq \Lc (\W(\tau)) - \frac{\eta}{2}  \tf{\nabla \Lc(\W(\tau))}^2 \\ 
    \end{split}
    \end{equation}
The inequality above also indicates that
\begin{equation}
    \sum_{\tau = 0}^{\infty} \tf{\nabla \Lc(\W(\tau))}^2 \leq \frac{2}{\eta} (\mathcal{L}(\W(0)) - \mathcal{L}^*)<\infty,~~~\text{and}~~~ \lim_{\tau \to \infty} \tf{\nabla \Lc(\W(\tau))}^2 = 0
\end{equation}
\end{proof}
\subsection{Proof of Lemma~\ref{lemma cvx}}
\begin{proof}

We first prove that $\Lc(\W)$ is convex. 
    Let $(\X, y)$ be an arbitrary pair of input sequence and label. Let $\vb(\W):=\Eb\W\xl$ and $v_k = \eb_k^\top \W \bar{\x}$ for $k \in [K]$ and let $m_k$ be the number of token ID $k$ inside input sequence $\X$. By Assumption \ref{assume loss} and \ref{assume iden}, we know that
    \begin{align}
       \ell(\vb):= \ell(\cb_{y}^\top \X^\top \sft{\X \W \bar{\x}}) = -\log\left(\frac{m_y\cdot e^{v_{y}}}{\sum_{k\in[K]} m_k\cdot e^{v_k}} \right) = \log\left(\sum_{k \in [K]} m_k\cdot e^{v_k}\right) - v_y-\log m_y.
   \end{align}
   % Since $\nabla^2\vb(\W)=0$, $\vb$ is convex. Next, it remains to 
   We first show that $\ell(\vb)$ is convex. 
   Let $\z \in \R^{K}$ be a vector such that the $k$th element of $\z$ is $z_k=m_k e^{v_{k}}$. Then, the Hessian matrix of $\ell(\vb)$ is as follows:
\begin{align}
    \nabla^2 \ell(\vb) = \frac{1}{(\boldsymbol{1}^\top \z)^2}\left((\boldsymbol{1}^\top \z) \text{diag}(\z) - \z \z^\top \right)
\end{align}
For any $\ub \in \R^K$, we obtain that 
\begin{align}\label{CSI}
    \ub^\top \nabla^2 \ell(\vb) \ub = \frac{1}{(\boldsymbol{1}^\top \z)^2} \left( \left(\sum_{k=1}^K z_k \right) \left(\sum_{k=1}^K u_k^2 z_k\right)  - \left(\sum_{k=1}^K u_k z_k \right)^2 \right) \geq 0  .
\end{align}
Since $\z_k>0$, $k\in[K]$, \eqref{CSI} follows from the Cauchy-Schwarz inequality $(\bal^\top \bal)(\bt ^\top \bt) \geq (\bal^\top \bt)^2$ applied to the vectors with $\alpha_i = u_i \sqrt{z_i}$ and $\beta_i = \sqrt{z_i}$. The equality condition holds $k \bal = \bt$ for $k \neq 0$. This means that $\ell(\vb)$ is convex. We know that $\Lc(\W)$ is the summation of $\ell(\vb)$ and $\vb$ is a linear transformation of $\W$. Combining these two facts implies that $\Lc(\W)$ is convex. 

Next, we will show that under Assumption~\ref{assume orth}, $\Lc(\W)$ is strongly convex on subspace $\Scf$. Following Definition~\ref{def finite correct}, let us define the subspace $\Scf^{ki}$ for $k \in [K], i \in [N_k]$ such that it is equal to the span of all matrices $(\eb_j - \bar\eb_i^{(k)}) \eb_k^\top$ for $j \in \Cc_i^{(k)}$. Then, we know that all of $\Scf^{ik}$ are orthogonal to each other by Assumption \ref{assume orth}, and their union results in $\Scf$. Assume that $\Lc(\W)$ is not strongly convex on $\Scf$. This means that there exist $\W_1, \W_2 \in \Scf$, $\tf{\W_2} > 0$ and $0 < \lambda < 1$ such that %if $0 < \lambda < C$, then we have
\begin{equation}\label{strongconvexityinverse}
    \Lc((1- \lambda) \W_1 + \lambda (\W_1 + \W_2)) = (1-\lambda )\Lc(\W_1) + \lambda \Lc(\W_1 + \W_2).
\end{equation}
We will show that $\tf{\Pi_{\Scf^{ik}} (\W_2)} = 0$ for all $i,k$. Let us first assume that there exist $\bar{i},\bar{k}$ such that $\tf{\Pi_{\Scf^{\bar{i}\bar{k}}}(\W_2)} > 0$ and let $\W_1^{\bar{i}\bar{k}} = \Pi_{\Scf^{\bar{i}\bar{k}}}(\W_1) $ and $\W_2^{\bar{i}\bar{k}} = \Pi_{\Scf^{\bar{i}\bar{k}}}(\W_2)$.  We can decompose $\W_2^{\bar{i} \bar{k}}$ in the following way:
\begin{align}\label{decompositionW2ik}
    \W_2^{\bar{i} \bar{k}} = \sum_{j \in \Cc_{\bar{i}}^{(\bar{k})}} \alpha_j (\eb_j - \bar{\eb}_{\bar i}^{(\bar{k})}) \eb_{\bar{k}}^{\top}.
\end{align}
Let $(\X_i, y_i)_{i=1}^m$ be all input sequence label pairs of $\bdata$ that induces an edge in $\Cc_{\bar{i}}^{(\bar{k})}$. For $i \in [m]$, let $\vb_i = \X_i \W_1^{\bar{i}\bar{k}} \eb_{\bar{k}}$, $\ell(\vb_i) = \ell(\cb_{y_i} \X_i^\top \sft{\X_i \W_1^{\bar{i}\bar{k}} \eb_{\bar{k}}})$, and $\ub \in \R^{K}$ such that $u_k = \eb_k^\top \W_2^{\bar{i}\bar{k}} \eb_{\bar{k}}$ for $k \in [K]$. Combining \eqref{strongconvexityinverse} and the fact that $\ell(\vb)$ is convex, we obtain
\begin{align}
    \ub^\top \nabla^2 \ell(\vb_i) \ub = 0 \qquad \forall i \in [m].
\end{align}
Combining the equality condition of Cauchy-Schwarz inequality and the fact that there exists a way to go between two nodes if they are in the same SCC, we obtain that $u_i = u_j$ for each $i, j \in \Cc_{\bar{i}}^{(\bar{k})}$ (Otherwise $\sum_{i}\ub^\top \nabla^2 \ell(\vb_i) \ub>0$). Utilizing \eqref{decompositionW2ik} and the fact that $u_i = \eb_i^\top \W_2^{\bar{i}\bar{k}} \eb_{\bar{k}}$, $\alpha_j = 0$ for all $j \in \Cc_{\bar{i}}^{(\bar{k})}$ is the only solution. This means that $\tf{\W_2^{\bar{i}\bar{k}}} = 0$, which is a contradiction. Therefore, $\Lc(\W)$ is strongly convex on $\Scf$.
\end{proof}
