# Supplementary material for: Mechanics of Next Token Prediction with Self-Attention
Source: arXiv:2403.08081 source file (2024-03-12)
Supplement: Supplementary file 5 [file lemmas.tex]

    % \section{TODOs}
    % \begin{itemize}
    %     \item Regularization Path for Theorem 1 and 2 
    %     \item Experiments: 
    %     \item $\Wf$ regularization path and proving $\Wf$ is finite 
        
    % \end{itemize}
    \section{Auxiliary Lemmas}
    \subsection{}
    \begin{lemma}\label{lemma reg wfin} Consider the same setting of Theorem~\ref{thm cyclic gd}. For any $\W\in\Scf$, there exists sufficiently large $R_{\W}$ such that for any $R\geq R_{\W}$
    \[
    \Lc(R\cdot\Wm+\Wf)<\Lc(R\cdot\Wm+\W).
    \]
\end{lemma}
\begin{proof}
    Let $\ab_i=\X_i(R\cdot\Wm)\xli$, $\bb^\st_i=\X_i\Wf\xli$, $\bb=\X_i\W\xli$, $\s^\st_i=\sft{\ab_i+\bb^\st_i}$, and $\s_i=\sft{\ab_i+\bb_i}$. Recap from \eqref{def erm loss}, we have that
    \[
    \Lc(R\cdot\Wm+\Wf)=\frac{1}{n}\sum_{i=1}^n\ell\left(\sum_{t\in\Oc_i}s^\st_{it}\right)\quad\text{and}\quad\Lc(R\cdot\Wm+\W)=\frac{1}{n}\sum_{i=1}^n\ell\left(\sum_{t\in\Oc_i}s_{it}\right).
    \]
    
    Following the similar analysis in the proof of Lemma~\ref{lemma reg orth dir}, and letting $\Lc_\st:=\min_{R\to\infty}\Lc(R\cdot\Wm+\Wf)$ which has been proven to be the optimal risk (see Theorem~\ref{thm cyclic gd}),  we prove $\Lc(R\cdot\Wm+\Wf)<\Lc(R\cdot\Wm+\W)$ by studying their loss distances to $\Lc_\st$.

    \begin{align*}
        &\sum_{t\in\Oc_i}s_{it}=\frac{\sum_{t\in\Oc_i}e^{a_{it}+b_{it}}}{\sum_{t\in[T_i]}e^{a_{it}+b_{it}}}=\frac{\sum_{t\in\Oc_i}e^{b_{it}}}{\sum_{t\in\Rc_i}e^{b_{it}}+\sum_{t\in\Rcb_i}e^{b_{it}-R}}\leq\frac{c_i}{d_i+e^{b_1-R}}\quad\text{for all~}i\in[n]\\
        &\sum_{t\in\Oc_i}s^\st_{it}=\frac{\sum_{t\in\Oc_i}e^{a_{it}+b^\st_{it}}}{\sum_{t\in[T_i]}e^{a_{it}+b^\st_{it}}}=\frac{\sum_{t\in\Oc_i}e^{b^\st_{it}}}{\sum_{t\in\Rc_i}e^{b^\st_{it}}+\sum_{t\in\Rcb_i}e^{b^\st_{it}-R}}\geq\frac{c^\st_i}{d^\st_i+Te^{b_2-R}}\quad\text{for all~}i\in[n]
    \end{align*}
    where $b_1=\min_{t\in\Rcb_i,i\in[n]}b_{it}$ and $b_2=\max_{t\in\Rcb_i,i\in[n]}b^\st_{it}+\log(T)$. 
    Consider loss function $\ell(u)=-\log(u)$, then
    \begin{align*}
        &-\log\left(\sum_{t\in\Oc_i}s_{it}\right)\geq-\log\left(\frac{c_i}{d_i+e^{b_1-R}}\right)=-\log\left(\frac{c_i}{d_i}\right)-\log\left(\frac{1}{1+e^{b_1-R}/d_i}\right)\geq\frac{1}{d_ie^{R-b_1}+1}-\log\left(\frac{c_i}{d_i}\right)\\
        &-\log\left(\sum_{t\in\Oc_i}s^\st_{it}\right)\leq-\log\left(\frac{c^\st_i}{d^\st_i+Te^{b_2-R}}\right)=-\log\left(\frac{c^\st_i}{d^\st_i}\right)-\log\left(\frac{1}{1+Te^{b_2-R}/d^\st_i}\right)\leq Te^{b_2-R}/d^\st_i-\log\left(\frac{c^\st_i}{d^\st_i}\right)
    \end{align*}

    Since we have that $\Lc_\st=\frac{1}{n}\sum_{i=1}^n\ell(\frac{c_i^\st}{d_i^\st})$, $\lim_{R\to\infty}\Lc(R\cdot\Wm+\W)>\Lc_\st$, and loss function $\ell(u)=-\log(u)$ is strictly decreasing. Then
    \[
    \frac{1}{n}\sum_{i=1}^n-\log\left(\frac{c_i}{d_i}\right)-\frac{1}{n}\sum_{i=1}^n-\log\left(\frac{c_i^\st}{d_i^\st}\right):=\delta(\W)\geq0.%\Longrightarrow\Pi_{i\in[n]}\left(\frac{c_i}{d_i}\right)<\Pi_{i\in[n]}\left(\frac{c^\st_i}{d^\st_i}\right).
    \]
    Finally, we obtain
    \begin{align*}
        \Lc(R\cdot\Wm+\W)-\Lc_\st&\geq\frac{1}{n}\sum_{i=1}^n\frac{1}{d_ie^{R-b_1}+1}+\frac{1}{n}\sum_{i=1}^n\left(-\log\left(\frac{c_i}{d_i}\right)-\log\left(\frac{c_i^\st}{d_i^\st}\right)\right)\\
        &=\frac{1}{n}\sum_{i=1}^n\frac{1}{d_ie^{R-b_1}+1}+\delta\\
        &\geq\frac{1}{n}\frac{1}{d_j\cdot e^{R-b_1}+1}+\delta\\
        \Lc(R\cdot\Wm+\Wf)-\Lc_\st&\leq\frac{1}{n}\sum_{i=1}^n Te^{b_2-R}/d^\st_i\leq \frac{Te^{b_2-R}}{\dmx^\st}.
    \end{align*}
    \yl{Then for any $\delta(\W)>0$, there exist $R_{\W}=O(\log(1/\delta))$ such that for any $R>R_{\W}$, $\Lc(R\cdot\Wm+\W)>\Lc(R\cdot\Wm+\Wf)$. Here, $O(\cdot)$ subsumes the constant dependencies. It completes the proof. }
\end{proof}

\begin{lemma}
    Consider the setting of Theorem~\ref{thm cyclic gd}. Define
    \[
    \Wf_R:=\arg\min_{\W}\Lc(R\cdot\Wm+\W).
    \]
    We have that for any $R>0$, $\tf{\Wf_R}<\infty$ and $\lim_{R\to\infty}\Wf_R=\Wf$.
\end{lemma}
\begin{proof}
    
\end{proof}
\begin{lemma} \label{lemma negcorr} Consider a cyclic dataset $\data$ following Definition~\ref{def acyc}, and let $\Wm$ be the SVM solution of \eqref{acyc svm}. Suppose Assumptions \ref{assume loss}, \ref{assume realizable} and \ref{assume same corr pred} hold, and suppose $\Wm$ is feasible. Then for all $\W \in \R^{d \times d}$, the training loss $\Lc(\W)$ obeys $\langle {\nabla \mathcal{L}(\W), \Wm} \rangle < 0$.
\end{lemma}
% \begin{lemma}
% Consider any dataset $\data$ under the same setting as in Lemma \ref{lemma negcorr}. Let $\Wm$ be the SVM solution of \eqref{graph svm}, and suppose $\Wm$ is feasible and $\Wm\neq0$. Then for all $\W\in\R^{d\times d}$, the training loss $\Lc(\W)$ obeys $\langle {\prj_{\Scf^\perp}(\nabla \mathcal{L}(\W)), \Wm} \rangle < 0$ and $\langle {\prj_{\Scf}(\nabla \mathcal{L}(\W)), \Wf} \rangle \leq 0$, where the equality holds only when $\prj_{\Scf}(\nabla \mathcal{L}(\W))=\Wf$.
% \end{lemma}

\begin{proof} 
Given dataset $\data=(\X_i,y_i)_{i=1}^n$, recap the problem 
\[ 
\Lc(\W)=\frac{1}{n}\sum_{i=1}^n \ell(\cb_{y_i}^\top\X_i^\top \sft{\X_i\W\xli}).
\]
Let 
\begin{equation}
    \bar{\hb}_i = \X_i\Wm \xli, \bgam_i = \X_i \cb_{y_i}, \text{ and } \hb_i =\X_i \W \xli
\end{equation}
 Recalling that the gradient evaluated at $\W$ is: 
\begin{equation}
        \nabla \mathcal{L}(\W) = \frac{1}{n} \sum_{i=1}^n \ell' \left(\bgam_i^\top \sft{\hb_i}\right) \X_i^{\top} \mathbb{S}'{(\hb_i)}\bgam_i \xli^{\top}.
\end{equation}
As a result,
\begin{equation} \label{eq:negcorr 2}
\begin{split}
    \left\langle {\nabla \mathcal{L}(\W), \Wm} \right\rangle 
    &= \frac{1}{n} \sum_{i=1}^n \ell' \left(\bgam_i^\top \sft{\hb_i}\right) 
    \langle {\X_i^{\top} \mathbb{S}'{(\hb_i)}\bgam_i \xli^{\top}, \Wm} \rangle \\ 
    &= \frac{1}{n} \sum_{i=1}^n \ell_i' \cdot \text{trace}\left( (\Wm)^{\top} \X_i^{\top} \mathbb{S}'{(\hb_i)}\bgam_i \xli^{\top} \right) \\ 
    &\stackrel{(a)}{=} \frac{1}{n} \sum_{i=1}^n \ell_i' \cdot \bar{\hb}_i^{\top} \mathbb{S}'{(\hb_i)}\bgam_i \\ 
    &= \frac{1}{n} \sum_{i=1}^n \ell'_i \cdot \bar{\hb}_i^{\top} (\text{diag}(\s_i) - \s_i\s_i^{\top} )\bgam_i \\ 
\end{split}
\end{equation}
where $\ell'_i \coloneqq \ell' \left(\bgam_i^\top \sft{\hb_i}\right), \s_i = \sft{\hb_i}$ and (a) utilizes $\text{trace}(\bb \ab^{\top}) = \ab^{\top}\bb$.

% \redp{By definition there exists $i$ such that $y \in \Cc_i$. The define the set $\Oc$ as follows:
% \begin{align}
%     \Oc := \{t | \Xs_t \in \Cc_i, t \in [T]\}
% \end{align}}
Since loss function $\ell$ is strictly decreasing (Assumption~\ref{assume loss}), we have $\ell'_i<0$ for all $i\in[n]$. In the following, we drop the subscript $i$ for simplicity and focus on the sequence $(\X,y)$, scores $\bgam=\X\cb_y$, and $\bar\hb=\X\Wm\bar\x$ and $\hb=\X\W\bar\x$. Define the relevant token indices as 
\[
\Oc:=\{t~\big|~\x_t=\eb_y,t\in[T]\}.
\]
Then following Assumption~\ref{assume same corr pred}, we have that $\bgam_t=\alpha+\beta$ for $t\in\Oc$ and $\bgam_t=\beta$ for $t\in\Ocb:=[T]-\Oc$. Then 
\begin{equation}
\begin{split}
    \bar{\hb}^{\top} (\text{diag}(\s) - \s\s^{\top})\bgam 
    &= \sum_{t = 1}^T \bar{\hb}_t\s_t\bgam_t - \sum_{t = 1}^T \bar{\hb}_t\s_t\sum_{t = 1}^T \s_t\bgam_t \\ 
    &= (\alpha+\beta)\sum_{t \in \Oc} \bar{\hb}_t\s_t+\beta\sum_{t \in \Ocb} \bar{\hb}_t\s_t  - \left(\sum_{t=1}^T \bar{\hb}_t\s_t\right)\left((\alpha+\beta)\sum_{t \in \Oc}\s_t+\beta\sum_{t \in \Ocb}\s_t\right) \\ 
    &= \alpha\left(\sum_{t \in \Oc} \bar{\hb}_t\s_t-\sum_{t=1}^T\bar\hb_t\s_t\sum_{t\in\Oc}\s_t\right)\\%+\beta\left(\sum_{t=1}^T \bar{\hb}_t\s_t  - \sum_{t=1}^T \bar{\hb}_t\s_t\right) \\ 
    &=\alpha\sum_{t\in\Oc}\s_t\left(\bar\hb_y-\sum_{t=1}^T\bar\hb_t\s_t\right)\\
    &=\alpha\sum_{t\in\Oc}\s_t\left(\sum_{t=1}^T\bar\hb_y\s_t-\sum_{t=1}^T\bar\hb_t\s_t\right)\\
    &=\alpha\sum_{t\in\Oc}\s_t\left(\sum_{t=1}^T(\bar\hb_y-\bar\hb_t)\s_t\right),
\end{split}
\end{equation}
where we set $\bar\hb_y=\eb_y^\top\Wm\bar\x$. Recall that $\Xs_t$ denotes the scalar token ID of $\x_t$. Then following \eqref{graph svm} where $\bar\x=\eb_k$, we have that for all $t\in[T]-\Oc$, 
\[
\bar\hb_y-\bar\hb_t\begin{cases}=0\quad\text{for all}\quad y\asymp \Xs_t \in\Gck\\
\geq 1\quad \text{for all}\quad y\not\asymp \Xs_t,~(y\rightarrow \Xs_t)\in\Gck\end{cases}.
\]
It results in that  $\bar{\hb}_i^{\top} (\text{diag}(\s_i) - \s_i\s_i^{\top})\bgam_i >0$, $i\in[n]$ for \eqref{acyc svm} and $\bar{\hb}_i^{\top} (\text{diag}(\s_i) - \s_i\s_i^{\top})\bgam_i \geq0$, $i\in[n]$ for \eqref{graph svm}. Next, we will show that for \eqref{graph svm}, there exists $i\in[n]$ such that $\bar{\hb}_i^{\top} (\text{diag}(\s_i) - \s_i\s_i^{\top})\bgam_i >0$. Otherwise $\Wm=0$.

Now suppose for all $i\in[n]$, $\bar{\hb}_i^{\top} (\text{diag}(\s_i) - \s_i\s_i^{\top})\bgam_i =0$, which means that within each sequences, all the nodes lie in the same SCC, and therefore, problem \eqref{graph svm} is built without the "$\geq1$" constraints, and the solution is $\Wm=0$, which is contradictory to our assumption. 

Combing these with \eqref{eq:negcorr 2} and given the fact that $\ell'_i<0$ and $\alpha>0$, we have that 
\[
\left\langle {\nabla \mathcal{L}(\W), \Wm} \right\rangle<0,
\]
which completes the proof.
\end{proof}

        \subsection{Proof of Loss Lemma \ref{le:loss}}
\begin{lemma} \label{le:loss}
    Under Assumption \ref{assume loss}, $\nabla \Lc(\W)$ is $L$-Lipschitz continuous, where $a_i = \|\cb_{y_i}\|\:\|\xli\|^2\|\X_i\|^3, b_i = M_0\|\cb_{y_i}\|\: \|\X_i\| + 3M_1$ for all $i \in [n]$
    \begin{equation} \label{eq:lwconst}
        L = \frac{1}{n}\sum_{i=1}^n a_i b_i
    \end{equation}
\end{lemma}
        Setting:
        \begin{equation}
            \begin{split}
            E, C &\in \R^{K\times d} \\ 
                \Lc(\Cb,\W) & =\frac{1}{n}\sum_{i=1}^n \ell(\cb_{y_i}^\top\X_i^\top \sft{\X_i\W\xli}). \\
                % \mathcal{L}(\W) &= \frac{1}{n}\sum_{i=1}^n \ell \left(\y_i^\top \X_i^\top \sft{\X_i\W \x_{T_i}}\right)
            \end{split}
        \end{equation}
    \begin{proof} Let 
\begin{equation}
    \bgam_i = X_i \cdot \cb_{y_i}, \quad \hb_i = \X_i\W\xli
\end{equation}
% \begin{equation}
%     \bgam_i = X_i \cdot \y_i, \quad \hb_i = \X_i\W\x_{T_i}
% \end{equation}

From Assumption \ref{assume loss}, $\ell: \R \to \R$ is differentiable. Therefore, the gradient at $\W$ is given by:
\begin{equation}\label{gradient}
    \nabla \mathcal{L}(\W) = \frac{1}{n} \sum_{i=1}^n \ell' \left(\bgam_i^\top \sft{\hb_i}\right) \X_i^{\top} \mathbb{S}'{(\hb_i)}\bgam_i \xli^{\top}
\end{equation} 
where 
\begin{equation}
    \mathbb{S}'(\hb_i) = \text{diag}(\sft{\hb}) - \sft{\hb}\sft{\hb}^{\top} \in \R^{T \times T}
\end{equation}
Note that
\begin{equation} \label{eq:sftnorm}
    \|\mathbb{S}'(\hb_i)\| \leq \tf{\mathbb{S}'(\hb_i)} \leq 1 
\end{equation}
As a result, for any $\W, \dot{\W} \in \R^{d \times d}, i \in [n]$, we have
\begin{equation} \label{eq:sftlip1}
    \| \mathbb{S}({\hb}_i) - \mathbb{S}(\dot{\hb_i})\|  \leq  \| \hb_i - \dot{\hb_i}\| \leq 
    \|\X_i\|\: \|\xli\| \: \tf{\W - \dot{\W}}
\end{equation}
where $\dot{h_i} = \X_i \dot{\W}\xli$.
Similarly, 
\begin{equation} \label{eq:sftlip2}
\begin{split}
    \tf{\mathbb{S}'(\hb_i) - \mathbb{S}'(\dot{\hb_i})} 
    & \leq
    \|\mathbb{S}(\hb_i) - \mathbb{S}(\dot{\hb_i})\| + 
    \tf{\sft{\hb_i}\sft{\hb_i}^{\top} -  \sft{\dot{\hb_i}}\sft{\dot{\hb_i}}^{\top}} \\ 
    & \leq 
    3 \|\X_i\|\: \|\xli\| \: \tf{\W - \dot{\W}}  
\end{split}
\end{equation}
Moreover, for any $\W, \dot{\W} \in \R^{d \times d}$, we have:
\begin{equation}
\begin{split} \label{eq:gradlip}
    \tf{\nabla \mathcal{L}(\W) - \nabla \mathcal{L}(\dot{\W})} 
        & \leq 
        \frac{1}{n} \sum_{i=1}^n \tf{\ell' \left(\bgam_i^\top \sft{\hb_i}\right) \X_i^{\top} \mathbb{S}'{(\hb_i)}\bgam_i \xli^{\top} - \ell' \left(\bgam_i^\top \sft{\dot{\hb}_i}\right) \X_i^{\top} \mathbb{S}'{(\dot{\hb}_i)}\bgam_i \xli^{\top}} \\ 
        & \leq 
        \frac{1}{n} \sum_{i=1}^n \tf{\X_i^{\top} \mathbb{S}'{(\hb_i)}\bgam_i \xli^{\top}} \: \big|\ell' \left(\bgam_i^\top \sft{{\hb}_i}\right) - \ell' \left(\bgam_i^\top \sft{\dot{\hb}_i}\right)\big|  \\
        & + 
        \frac{1}{n} \sum_{i=1}^n \big|\ell' \left(\bgam_i^\top \sft{\hb_i}\right)\big| \: \tf{\X_i^{\top} \mathbb{S}'{({\hb}_i)}\bgam_i \xli^{\top} - \X_i^{\top} \mathbb{S}'{(\dot{\hb}_i)}\bgam_i \xli^{\top}} \\ 
        & \leq 
        \frac{1}{n} \sum_{i=1}^n M_0 \|\bgam_i\|^2 \: \|\xli\| \: \|\X_i\| \: \| \sft{h_i} - \sft{\dot{h_i}}\|  \\
        & + 
        \frac{1}{n} \sum_{i=1}^n M_1 \|\bgam_i\| \: \|\xli\| \: \|\X_i\| \: \tf{\mathbb{S}'(h_i) - \mathbb{S}'(\dot{h_i})} \\  
\end{split}
\end{equation}
where the second inequality derives from $|ab - cd| \leq |d||a - c| + |a||b-c|$ and the third inequality uses Assumption \ref{assume loss} and (\ref{eq:sftnorm})
with $\z_{k} = \x_T$ which is the last token in the sequence $\X$.

Substituting (\ref{eq:sftlip1}) and (\ref{eq:sftlip2}) into (\ref{eq:gradlip}), we get 
\begin{equation*}
\begin{split}
    \tf{\nabla \mathcal{L}(\W) - \nabla \mathcal{L}(\dot{\W})} 
    & \leq \frac{1}{n} \sum_{i=1}^{n} \left(M_0 \|\bgam_i\|^2 \: \|\xli\|^2 \: \|\X_i\|^2 + 3M_1 \|\bgam_i\| \: \|\xli\|^2 \: \|\X_i\|^2 \right) \tf{\W - \dot{\W}} \\ 
    & \leq \frac{1}{n} \sum_{i=1}^{n} \left(M_0 \|\cb_{y_i}\|^2 \: \|\xli\|^2 \: \|\X_i\|^4 + 3M_1 \|\cb_{y_i}\| \: \|\xli\|^2 \: \|\X_i\|^3 \right) \tf{\W - \dot{\W}} \\ 
    & = \frac{1}{n} \sum_{i=1}^{n} \left(M_0 \|\cb_{y_i}\|^2 \: \|\xli\|^2 \: \|\X_i\|^4 + 3M_1 \|\cb_{y_i}\| \: \|\xli\|^2 \: \|\X_i\|^3 \right) \tf{\W - \dot{\W}} \\
    & = \frac{1}{n} \sum_{i=1}^{n}(M_0 \|\cb_{y_i}\|\:\|\X_i\| + 3M_1) \: \|\cb_{y_i}\| \: \|\xli\|^2 \: \|\X_i\|^3 \tf{\W - \dot{\W}} \\
    & = L \tf{\W - \dot{\W}}
\end{split}
\end{equation*}

where $L$ is defined in (\ref{eq:lwconst})
\end{proof}

\subsection{Proof of Reduction Lemmas}

\begin{lemma} Suppose Assumption~\ref{assume orth} holds. Recap the ERM problem $\Lc(\W) =\frac{1}{n}\sum_{i=1}^n \ell(\cb_{y_i}^\top\X_i^\top \sft{\X_i\W\xli})$. Split the $n$ inputs into $K$ subsets so that each subset ($\Ic_k$) contains the same last token ($\xli=\eb_k$), that is, $\Ic_k=\{i~|~\bar\x_i=\eb_k,i\in[n]\}$ where $\bigcup_{k=1}^K\Ic_k=[n]$, and let $n_k=|\Ic_k|$. Then define subproblems $\Lc_k(\W) =\frac{1}{n_k}\sum_{i\in\Ic_k} \ell(\cb_{y_i}^\top\X_i^\top \sft{\X_i\W\eb_k})$. 

Let $\Sc_k$ be the span of all matrices $\vb\eb_k^\top$ for any $\vb\in\R^d$, $k\in[K]$, and let $\Sc^\perp=\R^{d\times d}-\sum_{k=1}^K\Sc_k$ be the subspace that is orthogonal to $\Sc_k$, $k\in[K]$. Let $\W_k=\prj_{\Sc_k}\W$ and $\W^\perp=\prj_{\Sc^\perp}\W$ where $\prj$ denotes the subspace projection with respect to Euclidean distance. Then starting form any initialization $\W(0)$, we have that for any $\tau\geq0$,
\[
\W(\tau)=\sum_{k=1}\W_k(\tau)+\W^\perp(0),
\]
where $\W_k(0)=\prj_{\Sc_k}\W(0)$, $\W^\perp(0)=\prj_{\Sc^\perp}\W(0)$ and 
\begin{align}
    \text{GD on combined problem:}~~&\W(\tau+1)=\W(\tau)-\eta\nabla\Lc(\W(\tau))\\
    \text{GD on subproblems:}~~&\W_k(\tau+1)=\W_k(\tau)-\eta_k\nabla\Lc_k(\W_k(\tau)),~~~\eta_k=\frac{n_k}{n}\eta,~k\in[K],
\end{align}
Hence training a single model $\W$ with initialization $\W(0)$ and step size $\eta$ is equivalent to training $K$ separate models each with initialization $\W_k(0)$, step size $\eta_k<\eta$ and data from $\Ic_k$.

\end{lemma}
\begin{proof} For any $\W\in\R^{d\times d}$, let $\W_k=\prj_{\Sc_k}\W$. Following Assumption~\ref{assume orth}, subspaces $\Sc_k,k\in[K]$ and $\Sc^\perp$ are orthogonal. Then we can decompose $\W$ via
\[
\W=\sum_{k=1}^{K}\prj_{\Sc_k}\W+\W^\perp=\sum_{k=1}^K\W_k+\W^\perp.
\]
Since $\eb_1,\cdots,\eb_K$ are orthonormal vectors, we have $\W_k\eb_j=0$, for all $j\neq k$, and $\W^\perp\eb_k=0$ for all $k\in[K]$.

We first show that $\sft{\X_i\W\eb_k}=\sft{\X_i\W_k\eb_k}$ and $\sfp{\X_i\W\eb_k}=\sfp{\X_i\W_k\eb_k}$. 
\begin{align}
    \X_i\W\eb_k=\X_i\left(\sum_{k=1}^K\W_k+\W^\perp\right)\eb_k=\X_i\W_k\eb_k\Longleftrightarrow\sft{\X_i\W\eb_k}=\sft{\X_i\W_k\eb_k}.
\end{align}
Let $\s=\sft{\X_i\W\eb_k}=\sft{\X_i\W_k\eb_k}$, then we have
\begin{align}
    \sfp{\X_i\W\eb_k}=\diag{\s}-\s\s^\top=\sfp{\X_i\W_k\eb_k}.
\end{align}

Now, we are ready to prove our main results. 
Recap the loss 
\begin{align}
\Lc(\W) &=\frac{1}{n}\sum_{i=1}^n \ell(\cb_{y_i}^\top\X_i^\top \sft{\X_i\W\xli})\\
&=\frac{1}{n}\sum_{k\in[K]}\sum_{i\in\Ic_k}\ell(\cb_{y_i}^\top\X_i^\top \sft{\X_i\W\eb_k})\\
&=\frac{1}{n}\sum_{k\in[K]}\sum_{i\in\Ic_k}\ell(\cb_{y_i}^\top\X_i^\top \sft{\X_i\W_k\eb_k})\label{sfx proj}\\
&=\frac{1}{n}\sum_{k\in[K]}n_k\Lc_k(\W_k)
\end{align}
where \eqref{sfx proj} comes from the fact that $\sft{\X_i\W\eb_k}=\sft{\X_i\W_k\eb_k}$, and following \eqref{gradient}, let $\bgam_i=\X_i\cb_{y_i}$, then the gradient is written by
\begin{align}
\nabla \Lc(\W) &=\frac{1}{n}\sum_{i=1}^n \ell'(\bgam_i^\top\sft{\X_i\W\xli})\X_i^\top \sfp{\X_i\W\xli}\bgam_i\xli^\top\\
&=\frac{1}{n}\sum_{k\in[K]}\sum_{i\in\Ic_k}\ell'(\bgam_i^\top\sft{\X_i\W\eb_k})\X_i^\top \sfp{\X_i\W\eb_k}\bgam_i\eb_k^\top\\
&=\frac{1}{n}\sum_{k\in[K]}\sum_{i\in\Ic_k}\ell'(\bgam_i^\top\sft{\X_i\W_k\eb_k})\X_i^\top \sfp{\X_i\W_k\eb_k}\bgam_i\eb_k^\top\label{sfx grad proj}\\
&=\frac{1}{n}\sum_{k\in[K]}n_k\nabla\Lc_k(\W_k).
\end{align}
where \eqref{sfx grad proj} follows the fact that $\sft{\X_i\W\eb_k}=\sft{\X_i\W_k\eb_k}$ and $\sfp{\X_i\W\eb_k}=\sfp{\X_i\W_k\eb_k}$. What's more, we have 
\[
\nabla\Lc_k(\W_k)(\nabla\Lc_j(\W_j))^\top=0,~~~\text{for all}~~~j\in[K],j\neq k.
\]
Then given step size $\eta>0$, the gradient iteration at time $\tau$ is updated by
\begin{align}
\W(\tau+1)&=\W(\tau)-\eta\nabla\Lc(\W(\tau))\\
&=\sum_{k\in[K]}\W_k(\tau)+\W^\perp(\tau)-\sum_{k\in[K]}\eta\frac{n_k}{n}\nabla\Lc_k(\W_k(\tau))\\
&=\sum_{k\in[K]}\W_k(\tau)-\eta_k\nabla\Lc_k(\W_k(\tau))+\W^\perp(\tau)\\
&=\sum_{k\in[K]}\W_k(\tau+1)+\W^\perp(\tau),
\end{align}
where $\W_k(\tau)=\prj_{\Sc_k}\W(\tau)$, $\eta_k=\eta n_k/n$, and $\W^\perp(\tau)=\W^\perp(0)$. It proves that training a model with the whole dataset (with $n$ inputs) and step size $\eta$ is equivalent to training and composing $K$ separate models, each with inputs whose last token is labeled by $k$ ($\xli=\eb_k$), initialization $\W_k(0)=\prj_{\Sc}\W(0)$ and step size $\eta_k=\eta n_k/n$.
\end{proof}
    
We start by proving the associated SVM solution for data with the same last token will be a rank-$1$ solution. \redp{Based on this, we can then prove the general solution is a summation of $K$ rank-$1$ solution.}
    \begin{lemma}\label{le:red1}
Suppose all the input sequences in $\data$ end with the same token $\xli = \eb_{k}$ and Assumption \ref{assume orth} holds. Any optimal solution of \eqref{acyc svm} or \eqref{graph svm} is at most rank 1. More precisely, the row space of $\Wm$ lies within $span(\eb_{k})$.
\end{lemma}
\begin{proof}
    Suppose the contrary that the row space of $\Wm_{\diamond}$ does not lie within $\mathcal{S} = span(\eb_k)$. Let $\W = \prj_{\mathcal{S}}(\Wm_{\diamond})$ denote the projected matrix of $\Wm_{\diamond}$ on $\mathcal{S}$. Observe that $\W$ satisfied all SVM constraints since $\W \eb_k = \Wm_{\diamond}\eb_k$ due to Assumption \ref{assume orth}. As $\Wm_{\diamond} \neq \W$, we then obtain a contradiction by $\tf{\Wm_{\diamond}}^2 = \tf{\W}^2 + \tf{\Wm_{\diamond} - \W}^2 > \tf{\W}^2$ since $\Wm_{\diamond}$ is a optimal solution. 
\end{proof}

\begin{lemma}[Reduction Lemma]\label{le:red2}
    For a general dataset $\data$ and its next-token graphs $(\Gck)_{k=1}^K$, if Assumption \ref{assume orth} holds, solving the SVM optimization problem \eqref{acyc svm} or \eqref{graph svm} with input $\data$ is equivalent to simultaneously solving $K$ SVM problems with the input $\datak$ for $k \in [K]$ respectively. As a result, $\Wm$ can be written as:
    \begin{equation}
        \Wm = \sum_{k = 1}^{m} \Wm_k
    \end{equation}
    where $\Wm_k$ is the corresponding solution to the SVM problem with input $\datak$.
\end{lemma}
\begin{proof}
    Recall that for \eqref{acyc svm} we have: 
    \begin{align*}
        \Wm=\arg\min_{\W}\tf{\W}\quad\text{such that}\quad (\eb_i-\eb_j)\W\eb_k\geq 1\quad \text{for all}\quad(i\rightarrow j)\in\Gck, k\in[K]
    \end{align*}
    Following Lemma \ref{le:red1}, we know that the row space of $\Wm$ lies within $span(\{\eb_k\}_{k=1}^m)$. To proceed, we project $\Wm$ to the subspace of $\eb_k$ and obtain $\W_k = \prj_{\eb_k}(\Wm)$. Since $\eb_k^T\eb_\tau = 0$ for any $k \neq \tau, k, \tau \in [K]$ from Assumption \ref{assume orth}, we can decompose $\Wm$ as the following:
    \begin{equation*}
        \Wm = \sum_{k=1}^K \W_k
    \end{equation*}
    where $\W_k = \prj_{\eb_k}(\Wm)$.
    % \begin{equation}
    %     \left \langle \W_{k}, \W_{\tau} \right \rangle = 0
    % \end{equation}
    % where $k \neq \tau, k, \tau \in [K]$. 
    Then for the Forbeinus norm objective, we have
    \begin{equation}
        \Wm = \arg\min_W \tf{\W} = \arg \min_W \tf{\W}^2 = \arg \min_{W = \sum_{k} \W_k} \sum_{k=1}^K{\tf{\W_k}^2}
    \end{equation}
    Moreover, the assumption also indicates that $\W_k$ and $\W_{\tau}$ will not interfere with each other regarding the SVM constraints. Specifically, for the SVM constraints induced by $\datak \text{ or } \Gck, \forall k \in [K]$, we have 
    \begin{equation}
        \Wm \eb_k = \W_k \eb_k 
    \end{equation}
    as $\W_{\tau} \eb_k = 0$ for $\tau \neq k, \tau \in [K]$. As a result, optimizing $\Wm$ is equivalent to optimizing $\W_k$ according to the following sub-SVM problem. 
    \begin{align}\tag{Acyc-SVM-k}
    \Wm = \sum_{k=1}^m \Wm_k, \Wm_k = \arg\min_{\W_k}\tf{\W_k}\quad\text{such that}\quad (\eb_i-\eb_j)\W_k\eb_k\geq 1\quad \text{for all}\quad(i\rightarrow j)\in\Gck
    \end{align}
    Similarly, we can extend the results to the solution of \eqref{graph svm}. 
\end{proof}
\subsection{Proof of SCC Lemma}
\begin{lemma}\label{lemma scc}
Under Assumption \ref{assume scc}, given $\data$, there is at least one directed edge between nodes which are in the different SCCs, 

i.e., there exists some $k \in [K], y \Rightarrow j \in \Gck$, 

where $y$ is the label of some $\Xs$. This also indicates that the solution $\Wm$ to problem \eqref{graph svm} cannot be zero. 
% Moreover, this indicates that the solution $\Wm$ of \eqref{acyc svm} or \eqref{graph svm} is not zero. 
\end{lemma}

\begin{proof}
To proceed, consider an SCC $\Cck_i$ that does not contain the last token index $k$. From the definition of $\Gck$, we know that there exists a directed edge $y \to k$ where $y$ is the label of some $\Xs$ and $y \in \Cck_i$. Since $y$ and $k$ are in the different SCCs, this completes the first part of the proof. 
Moreover, observe that this directed edge creates a constraint that $(\eb_y - \eb_k)^{\top}\W \eb_k \geq 1 $ in the problem \eqref{graph svm}. Suppose the claim is wrong and that $\Wm$ is zero. This immediately leads to a contradiction with the SVM constraint. As a result, $\Wm$ is nonzero under Assumption \ref{assume scc}.

\end{proof}
